# Supplementary material for: Physics-inspired Equivariant Descriptors of Non-bonded Interactions
Source: arXiv:2308.13208 source file (2023-10-03)
Supplement: Supplementary file 1 [file si.pdf]

# Physics-inspired Equivariant Descriptors of Non-bonded Interactions
**Supplemental Material**

Kevin K. Huguenin-Dumittan,[1,*] Philip Loche,[1,*] Ni Haoran,[1] and Michele Ceriotti[1,†]

[1] *Laboratory of Computational Science and Modeling, IMX, École Polytechnique Fédérale de Lausanne, 1015 Lausanne, Switzerland*

## CONTENTS

S1 Multipole Expansion: Review and Extension S2
A Overview S2
B Multipole Expansion for Coulomb Potential S3
1. Key ingredient: Laplace Expansion of Coulomb Potential S3
2. Interior Charges S5
3. Exterior Charges S6
4. Inter-Regional Interaction Energy S7
C Extension of Multipole Expansion to General Inverse Power-Law Potential S7
1. Key ingredient: Laplace Expansion of General Power-Law Potential S7
2. Interior Charges S9
3. Exterior Charges S10
4. Inter-Regional Interaction Energy S10
D Remark On Conventions and Prefactors S11

S2 Physical Interpretation and Optimization of LODE Representation S11
A Overview of this section S11
B General Framework for Atomic Representations S11
C LODE for Coulombic Interactions S12
D Extension to Arbitrary Long-Range Descriptors S13
E Physical Interpretation and Optimizations for the Coulombic Case S14
F Physical Interpretation and Optimizations for General Exponents S15
G Building ML Models S16

S3 Similarities and Differences of the LODE Density with the actual Coulomb Potential S17
A Absence of SR-LR splitting S17
B Treatment of different chemical species S17

S4 Behavior of General Density Contribution Function S18
A Long-Range Limit S19
B Short-Range Limit S19
C Coulombic Special Case S19
D Why Gaussian Densities cannot be used in the general case S20

S5 Model Details for the Point-Charge Toy problem S20

S6 Computational details for the Dimer Dataset S20
A Reference energy calculations S20
B Empirical interaction exponents S20
C SOAP and LODE Hyperparameters S22
D Linear Models: Separate Dimer Classes S22
E Atomic Force Errors S22
F Test Errors for Different Training Cutoffs S23
G Energy Errors for Combined Linear Models Using Non-Charged Fragments S24
H Details of the Neural Network Models S24
I Absolute Eenergy Errors for Different Subsets S25

S7 Flexibility of power-law fits S25

References S27

---

* These two authors contributed equally.
† michele.ceriotti@epfl.ch

# S1. MULTIPOLE EXPANSION: REVIEW AND EXTENSION

## A. Overview

A key ingredient for our analysis is the multipole expansion from electrostatics. To summarize the general idea, let $\rho(\boldsymbol{r})$ be some density function that decays sufficiently fast as $r \to \infty$, in a sense that will be made more precise later on.

As shown in Fig. S1a, we split the density up into an interior part $\rho^<$ and exterior part $\rho^>$, each containing only the density inside / outside the cutoff radius $r_{\text{cut}}$, respectively. More formally, this can be written as

$$\rho^<(\boldsymbol{r}) = \begin{cases} \rho(\boldsymbol{r}) & r < r_{\text{cut}} \\ 0 & r \geq r_{\text{cut}} \end{cases}, \quad \rho^>(\boldsymbol{r}) = \begin{cases} 0 & r < r_{\text{cut}} \\ \rho(\boldsymbol{r}) & r \geq r_{\text{cut}}, \end{cases} \tag{S1}$$

where $r = |\boldsymbol{r}|$ and $r' = \|\boldsymbol{r}'\|$. For the rest of this document, we shall denote by $\boldsymbol{r}$ ($\boldsymbol{r}'$) a point inside (outside) the cutoff, meaning that we will always have $r < r_{\text{cut}}$ ($r' > r_{\text{cut}}$). In particular, $r < r'$ will always be true.

We begin by providing a general overview of the multipole expansion: Now that we have divided space into two regions (interior and exterior), the multipole expansion is a technique that can be used to study the potential generated by charges in one region evaluated in the other region. To be more specific, we will derive expressions for the following three quantities:

1. The "famous version": The "electrostatic" potential $V^<$ generated by the interior charges, evaluated at a point $\boldsymbol{r}'$ in the exterior region as shown in Fig. S1b and explicitly given by

$$V^<(\boldsymbol{r}') = \int_0^{r_{\text{cut}}} \mathrm{d}^3\boldsymbol{r}\, \frac{\rho^<(\boldsymbol{r})}{\|\boldsymbol{r} - \boldsymbol{r}'\|^p}, \tag{S2}$$

   where the integral runs over the entire interior region with $r < r_{\text{cut}}$.

2. The opposite of the above, i.e. the potential $V^>$ generated by the exterior charges, evaluated at a point $\boldsymbol{r}$ in the interior region as shown in Fig. S1c and explicitly given by

$$V^>(\boldsymbol{r}) = \int_{r_{\text{cut}}}^{\infty} \mathrm{d}^3\boldsymbol{r}'\, \frac{\rho^>(\boldsymbol{r}')}{\|\boldsymbol{r} - \boldsymbol{r}'\|^p}, \tag{S3}$$

   where the integral runs over the entire exterior region with $r' > r_{\text{cut}}$.

3. The "electrostatic" interaction energy between the two regions: it consists of interaction terms of the form $\frac{q_i q_j}{\|\boldsymbol{r}_i - \boldsymbol{r}_j'\|^p}$, where particle $i$ is from the interior and $j$ from the exterior region. In other words, it includes the inter-regional interactions but not the intra-regional ones. For the continuous charge densities treated here, this can be written as

$$E_{\text{int}} = \int_0^{r_{\text{cut}}} \mathrm{d}^3\boldsymbol{r} \int_{r_{\text{cut}}}^{\infty} \mathrm{d}^3\boldsymbol{r}'\, \frac{\rho^<(\boldsymbol{r})\rho^>(\boldsymbol{r}')}{\|\boldsymbol{r} - \boldsymbol{r}'\|^p}. \tag{S4}$$

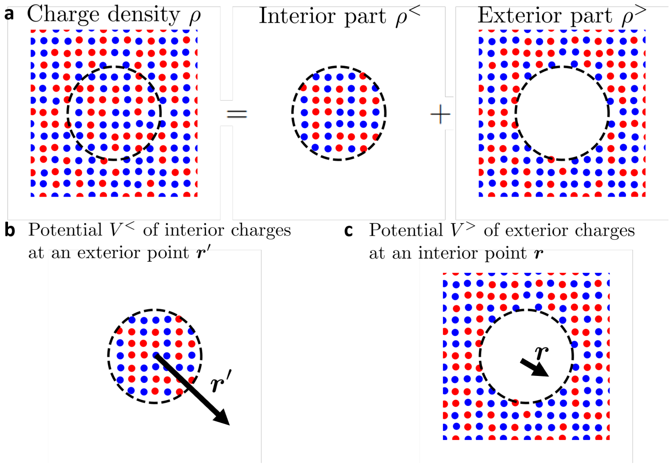


Figure S1. Visual representation of the various versions of the multipole expansion: a shows the splitting of a charge density into an interior and exterior part. b shows the "famous version" of the multipole expansion discussion in point 1. c shows the converse, in which the charges are outside and the potential is evaluated in the interior region.

The multipole expansion essentially provides a mathematically elegant way to express the three quantities defined in Eq. (S2), (S3) and (S4).

The separation into the two regions might at first seem arbitrary, but turns out to be a key ingredient: In Eq. (S2), for instance, we can observe that for the entire region of integration, we always have $r < r'$ since $\boldsymbol{r}'$ was specifically chosen to be a point in the exterior region $r' > r_{\text{cut}}$. This inequality will be essential to obtain a simple mathematical expression for the end result.

The most famous version of the multipole expansion that is discussed in many graduate level textbooks on electrodynamics deals with the first case, in which the charges are confined to some interior region [1], and is restricted to the Coulomb potential for which $p = 1$. The same derivation with tiny modifications also lead to the analogous results for the second (Eq. (S3)) and third (Eq. (S4)) cases. In fact, the proofs for all cases are quite simple once one knows one key intermediate result that is common to all three versions: the Laplace expansion of the Coulomb potential. A unified description of these for the Coulomb potential is discussed in section S1 B.

As part of this work, the multipole expansion was extended to arbitrary exponents $p$. The general case turns out to be more complicated than the Coulomb special case, the underlying reason being the fact that the Coulomb potential is a solution to the Laplace equation $\Delta\frac{1}{r} = 0$ for $r \neq 0$. This can be seen most directly by performing the multipole expansion in Cartesian coordinates. The analogous results for general exponents $p$ are discussed in section S1 C.

## B. Multipole Expansion for Coulomb Potential

### 1. *Key ingredient: Laplace Expansion of Coulomb Potential*

All variants of the multipole expansion are quite simple to derive once we understand a single key ingredient: the Laplace expansion of the Coulomb potential. In this subsection, we will first state the result and provide some intuition for why it is such an essential tool. For the more mathematically inclined readers, this is then followed by a sketch of the proof, but readers may feel free to skip this part and move on to the following subsections in which the Laplace expansion is used to derive the various versions of the multipole expansion.

**Lemma S1.1** (Laplace Expansion of Coulomb Potential)**.** *Let $\boldsymbol{r}, \boldsymbol{r}' \in \mathbb{R}^3$ such that $r < r'$. Then,*

$$\frac{1}{\|\boldsymbol{r} - \boldsymbol{r}'\|} = \sum_{l,m} \frac{4\pi}{2l+1} \frac{r^l}{r'^{l+1}} Y_l^m(\hat{\boldsymbol{r}}') Y_l^m(\hat{\boldsymbol{r}}), \tag{S5}$$

*where $\sum_{l,m}$ is a shorthand for $\sum_{l=0}^{\infty}\sum_{m=-l}^{l}$ and the functions $Y_l^m$ are the real spherical harmonics.*

The key idea is that we have managed to rewrite the the original expression, which depends on both $\boldsymbol{r}$ and $\boldsymbol{r}'$, into a form in which the two variables are separated, namely:

$$\frac{1}{\|\boldsymbol{r} - \boldsymbol{r}'\|} = \sum_{l,m} \frac{4\pi}{2l+1} \cdot \underbrace{\frac{1}{r'^{l+1}} Y_l^m(\hat{\boldsymbol{r}}')}_{\text{only depends on } \boldsymbol{r}'} \cdot \underbrace{r^l Y_l^m(\hat{\boldsymbol{r}}')}_{\text{only depends on } \boldsymbol{r}} . \tag{S6}$$

The radial dependencies (the factors of $r^l$ and $1/r'^{l+1}$) also explain why we need to split the charges into an interior and exterior part when we later discuss the full multipole expansion. For two general vectors $\boldsymbol{r}_1$ and $\boldsymbol{r}_2$, the Laplace expansion of $1/\|\boldsymbol{r}_1 - \boldsymbol{r}_2\|$ would contain factors of $r_{\text{min}}^l$ and $1/r_{\text{max}}^{l+1}$, where $r_{\text{max}}$ ($r_{\text{min}}$) is the larger (smaller) of the two radii $r_1$ and $r_2$. By dividing the charges into an interior and exterior region, we will always have $r < r'$ and thus $r_{\text{min}} = r$, $r_{\text{max}} = r'$. Otherwise, one would need to mix factors of $\frac{r^l}{r'^{l+1}}$ and $\frac{r'^l}{r^{l+1}}$, leading to significantly more complicated final expressions.

For readers not as familiar with the *real* spherical harmonics, these are essentially the same functions as the complex counterparts more often encountered in the mathematical literature. They are analogous to solutions of the differential equation $f'' = -f$, two commonly used forms being $f(x) = Ae^{ix} + Be^{-ix}$ or $f(x) = C\cos x + D\sin x$. The complex spherical harmonics correspond to the exponential solutions $e^{\pm ix}$, and tend to be easier to work with in proofs, while the trigonometric functions are real-valued, and hence favorable in applications in which the target function $f$ is known to be real. For this reason and for simpler notation, we use the real form, but all results would remain essentially the same with complex spherical harmonics, the only difference being that half of the spherical harmonics would need to be replaced by their complex conjugate.

We devote the rest of this subsection to the proof of the Laplace expansion. It is not required to understand this proof to get to the multipole expansion in the next subsection.

*Proof.* The proof consists of three steps. The first one only requires relatively elementary algebra, while the other two will require some knowledge about special functions (Legendre polynomials and spherical harmonics). We begin by writing the left hand side explicitly in terms of the moduli $r, r'$ as well as the angle $\gamma$ between the vectors $\boldsymbol{r}$ and $\boldsymbol{r}'$,

$$\frac{1}{\|\boldsymbol{r}-\boldsymbol{r}'\|} = \frac{1}{((\boldsymbol{r}-\boldsymbol{r}')^2)^{\frac{1}{2}}} = \frac{1}{(r^2+r'^2-2rr'\cos\gamma)^{\frac{1}{2}}} = \frac{1}{r'\left(\left(\frac{r}{r'}\right)^2+1-2\left(\frac{r}{r'}\right)\cos\gamma\right)^{\frac{1}{2}}}, \tag{S7}$$

where we pulled out a factor of $r'$ in the last step, and the angular part can be explicitly computed as $\cos\gamma = \hat{\boldsymbol{r}}\cdot\hat{\boldsymbol{r}}'$.

For the second step, we use an identity involving Legendre polynomials in terms of a generating function, namely

$$\frac{1}{(1-2cx+x^2)^{\frac{1}{2}}} = \sum_{l=0}^{\infty} P_l(c)x^l \tag{S8}$$

for any $x, c \in \mathbb{R}$ with $|c| < 1$ and $|x| < 1$. In fact, this equation can be used to define the Legendre polynomials in the first place. We can use this identity with $x = r/r'$ and $c = \cos\gamma = \hat{\boldsymbol{r}}\cdot\hat{\boldsymbol{r}}'$, which leads us to

$$\frac{1}{\|\boldsymbol{r}-\boldsymbol{r}'\|} = \frac{1}{r'}\frac{1}{\left(1-2\left(\frac{r}{r'}\right)(\hat{\boldsymbol{r}}\cdot\hat{\boldsymbol{r}}')+\left(\frac{r}{r'}\right)^2\right)^{\frac{1}{2}}} \tag{S9}$$

$$= \frac{1}{r'}\sum_{l=0}^{\infty} P_l(\hat{\boldsymbol{r}}\cdot\hat{\boldsymbol{r}}')\frac{r^l}{r'^l} = \sum_{l=0}^{\infty} P_l(\hat{\boldsymbol{r}}\cdot\hat{\boldsymbol{r}}')\frac{r^l}{r'^{l+1}}. \tag{S10}$$

Note that at this point, we have managed to separate the radial dependences with respect to $r$ and $r'$, but not yet the angular part.

Thus, for the third and final step, we will use the spherical harmonics addition theorem, which connects the spherical harmonics to the Legendre polynomials:

$$P_l(\hat{\boldsymbol{r}}\cdot\hat{\boldsymbol{r}}') = \sum_{m=-l}^{l} \frac{4\pi}{2l+1} Y_l^m(\hat{\boldsymbol{r}}')Y_l^m(\hat{\boldsymbol{r}}) \tag{S11}$$

for any two unit vectors $\hat{\boldsymbol{r}}$ and $\hat{\boldsymbol{r}}'$. Note that this theorem is typically derived using the complex form of the spherical harmonics, in which case the first spherical harmonic is replaced by the complex conjugate. Extending this theorem to real spherical harmonics is then straight-forward using the fact that the conversion between real and complex spherical harmonics is a unitary transformation.

With this step, we have now separated the angular dependence with respect to $\hat{\boldsymbol{r}}$ and $\hat{\boldsymbol{r}}'$. Using this, we finally obtain the desired result

$$\frac{1}{\|\boldsymbol{r}-\boldsymbol{r}'\|} = \sum_{l,m} \frac{4\pi}{2l+1}\frac{r^l}{r'^{l+1}} Y_l^m(\hat{\boldsymbol{r}}')Y_l^m(\hat{\boldsymbol{r}}). \tag{S12}$$

For completeness, the analogous result with complex spherical harmonics would be

$$\frac{1}{\|\boldsymbol{r}-\boldsymbol{r}'\|} = \sum_{l,m} \frac{4\pi}{2l+1}\frac{r^l}{r'^{l+1}} Y^{*m}_{\mathrm{complex},l}(\hat{\boldsymbol{r}}')Y^{m}_{\mathrm{complex},l}(\hat{\boldsymbol{r}}). \tag{S13}$$

□

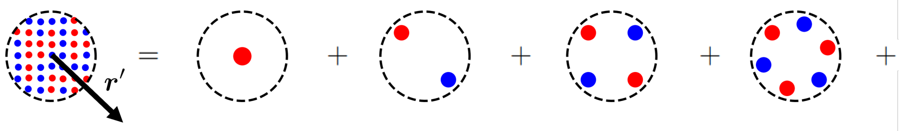


Figure S2. Visual representation of the interior multipole expansion. The potential generated by the interior charges can be decomposed into terms of increasing angular frequencies here illustrated for the first four ($l = 0, 1, 2, 3$) terms.

### 2. *Interior Charges*

We have now completed the most challenging part of the derivation, and are well-prepared to easily prove the multipole expansion theorems for the Coulomb potential. We begin by discussing the most well-known version of the Coulomb potential, which is discussed in many textbooks on electrodynamics [1] and is illustrated in Fig. S2.

**Theorem S1.2.** *Let $\rho^<$ be a localized charge density which is entirely contained within a cutoff radius $r_{\text{cut}}$. The resulting electrostatic potential $V^<(\boldsymbol{r}')$ evaluated at some point $\boldsymbol{r}'$ outside of the cutoff is given by*

$$V^<(\boldsymbol{r}') = \sum_{lm} M^<_{lm} \frac{1}{r'^{l+1}} Y^m_l(\hat{\boldsymbol{r}}'), \tag{S14}$$

*with coefficients*

$$M^<_{lm} = \frac{4\pi}{2l+1} \int_0^{r_{\text{cut}}} \mathrm{d}^3\boldsymbol{r}\, r^l Y^m_l(\hat{\boldsymbol{r}}) \rho^<(\boldsymbol{r}). \tag{S15}$$

The coefficients $M_{lm}$ are called **(interior) multipole moments** and completely characterize the potential in the exterior region. The first term with $l = 0$ is called the monopole term and generates a spherically symmetric potential decaying as $1/r$. The prefactor $M^<_{00}$ simply corresponds to the total charge. The second term with $l = 1$ is called the dipole term and generates a potential decaying as $1/r^2$. It represents the first correction to the spherically symmetrical approximation. More generally, as shown in Fig. S2, the multipole expansion can be thought of as a Fourier-like expansion of $\rho^<$ into angular frequency components. The term with an angular frequency $l$ leads to a potential decaying as $1/r^{1+l}$, showing that terms with high $l$ become less and less important as $r \to \infty$.

*Proof.* From the superposition principle, the electrostatic potential generated by $\rho^<$ is given by

$$V^<(\boldsymbol{r}') = \int_0^{r_{\text{cut}}} \mathrm{d}^3\boldsymbol{r}\, \frac{\rho^<(\boldsymbol{r})}{\|\boldsymbol{r} - \boldsymbol{r}'\|}. \tag{S16}$$

Since $r' > r_{\text{cut}}$, we have $r < r'$ in the entire domain of integration. This allows us to use the Laplace expansion of the Coulomb potential $\frac{1}{\|\boldsymbol{r}-\boldsymbol{r}'\|} = \sum_{l,m} \frac{4\pi}{2l+1} \frac{r^l}{r'^{l+1}} Y^m_l(\hat{\boldsymbol{r}}) Y^m_l(\hat{\boldsymbol{r}}')$ (Lemma (S5)) to write

$$V^<(\boldsymbol{r}') = \int_0^{r_{\text{cut}}} \mathrm{d}^3\boldsymbol{r}\, \rho^<(\boldsymbol{r}) \sum_{l,m} \frac{4\pi}{2l+1} \frac{r^l}{r'^{l+1}} Y^m_l(\hat{\boldsymbol{r}}) Y^m_l(\hat{\boldsymbol{r}}'). \tag{S17}$$

Assuming that $\rho^<$ is continuous on the entire interior domain (including the boundary), it is permissible to interchange the order of summation and integration from Fubini's theorem, which leads to

$$V^<(\boldsymbol{r}') = \sum_{l,m} \underbrace{\frac{4\pi}{2l+1} \int_0^{r_{\text{cut}}} \mathrm{d}^3\boldsymbol{r}\, \rho^<(\boldsymbol{r}) r^l Y^m_l(\hat{\boldsymbol{r}})}_{=:M_{lm}} \frac{1}{r'^{l+1}} Y^m_l(\hat{\boldsymbol{r}}') = \sum_{l,m} M^<_{lm} \frac{1}{r'^{l+1}} Y^m_l(\hat{\boldsymbol{r}}') \tag{S18}$$

with multipole moment

$$M^<_{lm} = \int_0^{r_{\text{cut}}} \mathrm{d}^3\boldsymbol{r}\, r^l Y^m_l(\hat{\boldsymbol{r}}) \rho^<(\boldsymbol{r}). \tag{S19}$$

This is the desired result, in which the exterior potential is written as a series in varying angular and radial dependence. □

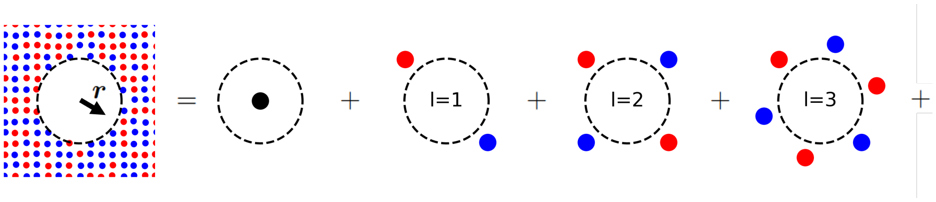


Figure S3. Visual representation of the exterior multipole expansion. The potential generated by the exterior charges can be decomposed into terms of increasing angular frequencies here illustrated for $l = 0, 1, 2, 3$ corresponding to the monopole, dipole, quadrupole and octupole terms.

### 3. *Exterior Charges*

We can now flip the roles between the exterior and interior regions: the charges are now outside, and we wish to compute the potential generated by these in the interior region. The result is analogous to the previous case, except that all factors of $r^l$ and $1/r'^l$ switch roles.

**Theorem S1.3.** *Let $\rho^>$ be a charge density which is entirely contained outside of a cutoff radius $r_{\mathrm{cut}}$. The resulting electrostatic potential $V^>(\boldsymbol{r})$ evaluated at some point $\boldsymbol{r}$ inside of the cutoff is given by*

$$V^>(\boldsymbol{r}) = \sum_{lm} M^>_{lm} r^l Y_l^m(\hat{\boldsymbol{r}}), \tag{S20}$$

*with coefficients*

$$M^>_{lm} = \frac{4\pi}{2l+1} \int_{r_{\mathrm{cut}}}^{\infty} \mathrm{d}^3\boldsymbol{r}' \, \frac{1}{r'^{l+1}} Y_l^m(\hat{\boldsymbol{r}}') \rho^>(\boldsymbol{r}'). \tag{S21}$$

The coefficients $M^>_{lm}$ will be called **exterior multipole moments** in this work. As for the interior version, this can be interpreted as a decomposition of the exterior charge density $\rho^>$ into (angular) frequency components as is illustrated in Fig. S3.

*Proof.* The proof follows along the exact same lines as the previous version, except that $r$ and $r'$ switch roles. From the superposition principle, the potential generated by the exterior charges is given by

$$V^>(\boldsymbol{r}) = \int_{r_{\mathrm{cut}}}^{\infty} \mathrm{d}^3\boldsymbol{r}' \, \frac{\rho^>(\boldsymbol{r}')}{\|\boldsymbol{r} - \boldsymbol{r}'\|}, \tag{S22}$$

assuming that the charge density $\rho^>$ decays sufficiently quickly for the integral to be well-defined. Using the Laplace expansion of the Coulomb potential (Eq. S5), we obtain

$$V^>(\boldsymbol{r}) = \int_{r_{\mathrm{cut}}}^{\infty} \mathrm{d}^3\boldsymbol{r}' \, \rho^>(\boldsymbol{r}') \sum_{l,m} \frac{4\pi}{2l+1} \frac{r^l}{r'^{l+1}} Y_l^m(\hat{\boldsymbol{r}}') Y_l^m(\hat{\boldsymbol{r}}). \tag{S23}$$

It is permissible to interchange the order of summation and integration if $rho^>$ decays sufficiently quickly. Thus,

$$V^>(\boldsymbol{r}) = \sum_{l,m} \underbrace{\frac{4\pi}{2l+1} \int_{r_{\mathrm{cut}}}^{\infty} \mathrm{d}^3\boldsymbol{r}' \, \frac{1}{r'^{l+1}} Y_l^m(\hat{\boldsymbol{r}}') \rho^>(\boldsymbol{r}')}_{=:M^>_{lm}} r^l Y_l^m(\hat{\boldsymbol{r}}) = \sum_{l,m} M^>_{lm} r^l Y_l^m(\hat{\boldsymbol{r}}) \tag{S24}$$

with coefficients

$$M^>_{lm} = \frac{4\pi}{2l+1} \int_{r_{\mathrm{cut}}}^{\infty} \mathrm{d}^3\boldsymbol{r}' \, \frac{1}{r'^{l+1}} Y_l^m(\hat{\boldsymbol{r}}') \rho^<(\boldsymbol{r}'). \tag{S25}$$

This is the desired result, in which the interior potential is written as a series in angular and radial dependence. □

### 4. Inter-Regional Interaction Energy

We now discuss the third and final useful result that can be derived using the same mathematical methods: the "inter-regional" electrostatic interaction energy $E_{\text{int}}$ between the charges in the two regions. More formally, let $\rho^<$ and $\rho^>$ be two charge densities that are confined to the interior / exterior region. The total electrostatic interaction energy $E_{\text{int}}$ between the interior and exterior charges (not including the interactions between charges in the same region) is given by

$$E_{\text{int}} = \int_0^{r_{\text{cut}}} \mathrm{d}^3\boldsymbol{r} \int_{r_{\text{cut}}}^{\infty} \mathrm{d}^3\boldsymbol{r}' \, \frac{\rho^<(\boldsymbol{r})\rho^>(\boldsymbol{r}')}{\|\boldsymbol{r}-\boldsymbol{r}'\|}. \tag{S26}$$

Obtaining a multipolar expression for this interaction energy will be useful to obtain a physical interpretation of ML models that are built on top of the LODE features.

**Theorem S1.4.** *The electrostatic interaction energy $E_{\text{int}}$ between the interior charges $\rho^<$ and exterior charges $\rho^>$ can be computed as*

$$E_{\text{int}} = \sum_{lm} \frac{2l+1}{4\pi} M^>_{lm} M^<_{lm}, \tag{S27}$$

*where $M^>_{lm}$ and $M^<_{lm}$ are the exterior and interior multipole moments defined in the two previous subsections S1 B 3 and S1 B 2, respectively.*

*Proof.* The proof should be straight-forward to anyone who has followed the proofs of the two previous versions of the multipole expansion. We start from

$$E_{\text{int}} = \int_0^{r_{\text{cut}}} \mathrm{d}^3\boldsymbol{r} \int_{r_{\text{cut}}}^{\infty} \mathrm{d}^3\boldsymbol{r}' \, \frac{\rho^<(\boldsymbol{r})\rho^>(\boldsymbol{r}')}{\|\boldsymbol{r}-\boldsymbol{r}'\|}. \tag{S28}$$

and rewrite $1/\|\boldsymbol{r}-\boldsymbol{r}'\|$ using the Laplace expansion of the Coulomb potential (Eq. (S5)). Then, after interchanging the order of the summation over $l, m$ and the two integrals, all factors containing $\boldsymbol{r}$ and $\boldsymbol{r}'$ are grouped together, leading to the desired result. □

## C. Extension of Multipole Expansion to General Inverse Power-Law Potential

We now extend this analysis to exponents other than $p = 1$. Just as before, we wish to derive three versions of the multipole expansion, corresponding to the three equations (S2) for interior charges, (S3) for exterior charges and (S4) for the interaction energy between the two regions. The key ingredient will be the generalization of the Laplace expansion of the Coulomb potential, discussed in section S1 B 1, to the general case. All variants of the multipole expansion will then follow in a straight-forward manner.

Note that different generalizations of the multipole expansion for general exponents have been proposed in the past, either based on the use of Cartesian coordinates or modified spherical harmonics. These methods, however, are less suitable for many ML applications in which we require a more systematic expansion in terms of the (usual) spherical harmonics due to symmetry reasons.

### 1. Key ingredient: Laplace Expansion of General Power-Law Potential

What made the Laplace expansion of the Coulomb potential so powerful was the fact that the expression $1/\|\boldsymbol{r}-\boldsymbol{r}'\|$ could be written in a way that provided a separation of the $\boldsymbol{r}$ and $\boldsymbol{r}'$ dependence. Thus, in order to generalize the mutipole expansion to arbitrary $1/r^p$ potentials, we need to derive an analogous expansion of $1/\|\boldsymbol{r}-\boldsymbol{r}'\|^p$. We begin by stating this generalized result and provide some intuition. As before, readers can feel free to skip the proof and continue to the next subsection, in which this lemma is used to prove the actual multipole expansion theorems.

**Lemma S1.5.** *Let $\boldsymbol{r}, \boldsymbol{r}' \in \mathbb{R}^3$ such that $r < r'$ and $p \in \mathbb{R}_+$. Then,*

$$\frac{1}{\|\boldsymbol{r}-\boldsymbol{r}'\|^p} = \sum_{nlm} \frac{4\pi}{2l+1} A^p_{n,l} \frac{r^{l+2n}}{r'^{p+l+2n}} Y^m_l(\boldsymbol{r}') Y^m_l(\boldsymbol{r}), \tag{S29}$$

*where $\sum_{nlm}$ is a shorthand for $\sum_{n=0}^{\infty}\sum_{l=0}^{\infty}\sum_{m=-l}^{l}$ and $A^p_{n,l}$ are suitable coefficients.*

Compared to the special case of $p = 1$ presented in Eq. (S5), we observe that the general version is more complex: it requires a sum over an additional index $n$, rather than just $l, m$. This is what makes all potentials with $p \neq 1$ qualitatively different from the Coulomb potential. As briefly mentioned before, $p = 1$ is special because applying the (three-dimensional) Laplace operator to $1/r$, we obtain $\Delta 1/r = 0$ for $r \neq 0$. It is, from a deeper point of view, this fact that eliminates all coefficients other than those where $n = 0$ in the Coulombic case.

*Proof.* The proof is similar to the one of Lemma S5, except that there is one extra step that leads to the more complicated multipole expansion also requiring a sum over $n$. The first step again uses simple algebra to rewrite the denominator as

$$\frac{1}{\|\boldsymbol{r}-\boldsymbol{r}'\|^p} = \frac{1}{(r^2 + r'^2 - 2rr'\cos\gamma)^{\frac{p}{2}}} = \frac{1}{r'^p\left(\left(\frac{r}{r'}\right)^2 + 1 - 2\left(\frac{r}{r'}\right)\cos\gamma\right)^{\frac{p}{2}}}, \tag{S30}$$

where $\cos\gamma = \hat{\boldsymbol{r}} \cdot \hat{\boldsymbol{r}}'$ is the angle between $\boldsymbol{r}$ and $\boldsymbol{r}'$.

For the next step, we will use a set of special functions called Gegenbauer polynomials (also known as ultraspherical polynomials), which are a generalization of Legendre polynomials. These obey the relation

$$\frac{1}{(1-2cx+x^2)^{p/2}} = \sum_{q=0}^{\infty} C_q^{p/2}(c)x^q. \tag{S31}$$

for any $x, c \in \mathbb{R}$ with $|c| < 1$ and $|x| < 1$ (alternatively, one could use this as a way to define the Gegenbauer polynomials in terms of a generating function). Note that for $p = 1$, the Gegenbauer polynomials $C_q^{1/2}$ reduce to the Legendre polynomials. We can use this identity with $x = r/r'$ and $c = \cos\gamma = \hat{\boldsymbol{r}} \cdot \hat{\boldsymbol{r}}'$, which leads us to

$$\frac{1}{\|\boldsymbol{r}-\boldsymbol{r}'\|^p} = \sum_{q=0}^{\infty} C_q^{p/2}(\hat{\boldsymbol{r}} \cdot \hat{\boldsymbol{r}'}) \frac{r'^q}{r^{p+q}}. \tag{S32}$$

Note that we have called the index of summation $q$ rather than $l$, for reasons that we will now explain.

In our application, we require a form of the multipole expansion that is written in terms of the spherical harmoncis functions $Y_l^m$. Thus, we need to find a way to express $C_q^{p/2}$ in terms of spherical harmonics. While no direct such relation is known to the authors, we can exploit the fact that Gegenbauer polynomials share many similarities to the Legendre polynomials: for all $p > 0$, $C_q^{p/2}$ is a polynomial of degree $q$. If $q$ is even (odd), then the function $C_q^{p/2}$ is even (odd) as well. Thus, using the analogous properties of the Legendre polynomials, we can see that there must exist some coefficients $\tilde{A}_{q,l}^p$ that allow us to express $C_q^{p/2}$ as a linear combination of Legendre polynomials $P_l$

$$C_q^{p/2} = {\sum_l}' \tilde{A}_{q,l}^p P_l, \tag{S33}$$

where the prime in the summation indicates that $l$ runs over $l = q, q-2, q-4, \ldots$ up to 0 or 1 depending on whether $q$ is even or odd due to the parity of both $P_l$ and $C_q$. We thus obtain

$$\frac{1}{\|\boldsymbol{r}-\boldsymbol{r}'\|^p} = \sum_{q=0}^{\infty} {\sum_l}' \tilde{A}_{q,l}^p P_l(\hat{\boldsymbol{r}} \cdot \hat{\boldsymbol{r}'}) \frac{r'^q}{r^{p+q}}. \tag{S34}$$

We can already observe a key difference to the electrostatic special case: For the Coulomb potential, the term decaying as $1/r^{1+l}$ only had an angular dependence of the form $P_l$, while for general $p$, the term decaying as $1/r^{p+q}$ requires multiple angular terms $P_l$ with $l = q, q-2, \ldots$ and so on. Equivalently, and more conveniently for our application, we can group together all terms that belong to the same value of $l$ and say that the term with an angular dependence of $P_l$ has radial dependence $1/r^{p+q}$ for $q = l, l+2, l+4, \ldots$. This can be reparametrized as $q = l + 2n$ for $n = 0, 1, 2, \ldots$. Thus, we obtain the general relation

$$\sum_{q=0}^{\infty} \sum_{l=q,q-2,\ldots} f(q,l) = \sum_{l=0}^{\infty}\sum_{n=0}^{\infty} f(l+2n, l) \tag{S35}$$

which can be applied to our case to yield

$$\frac{1}{\|\boldsymbol{r}-\boldsymbol{r}'\|^p} = \sum_{l=0}^{\infty}\sum_{n=0}^{\infty} \tilde{A}_{l+2n,l}^p P_l(\hat{\boldsymbol{r}} \cdot \hat{\boldsymbol{r}'}) \frac{r'^{l+n}}{r^{p+l+n}} =: \sum_{l=0}^{\infty}\sum_{n=0}^{\infty} A_{n,l}^p P_l(\hat{\boldsymbol{r}} \cdot \hat{\boldsymbol{r}'}) \frac{r'^{l+n}}{r^{p+l+n}}, \tag{S36}$$

where for convenience, we have re-indexed the coefficients $\tilde{A}^p_{l+2n}$ as $A^p_{n,l}$.

Finally, we can again use the spherical harmonics addition theorem

$$P_l(\hat{\boldsymbol{r}} \cdot \hat{\boldsymbol{r}}') = \sum_{m=-l}^{l} \frac{4\pi}{2l+1} Y_l^m(\hat{\boldsymbol{r}}') Y_l^m(\hat{\boldsymbol{r}}) \tag{S37}$$

to obtain the final expression

$$\frac{1}{\|\boldsymbol{r} - \boldsymbol{r}'\|^p} = \sum_{nlm} \frac{4\pi}{2l+1} A^p_{n,l} \frac{r^{l+2n}}{r'^{p+l+2n}} Y_l^m(\boldsymbol{r}') Y_l^m(\boldsymbol{r}) \tag{S38}$$

which concludes the proof. □

### 2. Interior Charges

We can now discuss the three versions of the multipole expansion for general exponent $p$. As for the Coulombic case, the most challenging part of the derivation is the Laplace expansion in Eq. (S29). If we accept this result, deriving the multipole expansion is just a simple extra step consisting of regrouping terms.

**Theorem S1.6.** *Let $\rho^<$ be a localized charge density which is entirely contained within a cutoff radius $r_{\text{cut}}$. The resulting "electrostatic" (inverse power-law) potential $V^<(\boldsymbol{r}')$ with exponent $p$ evaluated at some point $\boldsymbol{r}'$ outside of the cutoff is given by*

$$V^<(\boldsymbol{r}') = \sum_{nlm} M^<_{nlm} \frac{1}{r'^{p+l+2n}} Y_l^m(\hat{\boldsymbol{r}}'), \tag{S39}$$

*with coefficients*

$$M^<_{nlm} = \frac{4\pi}{2l+1} A^p_{n,l} \int_0^{r_{\text{cut}}} \mathrm{d}^3\boldsymbol{r}\, r^{l+2n} Y_l^m(\hat{\boldsymbol{r}}) \rho^<(\boldsymbol{r}), \tag{S40}$$

*and where $\sum_{nlm}$ is a shorthand for $\sum_{n=0}^{\infty} \sum_{l=0}^{\infty} \sum_{m=-l}^{l}$.*

*Proof.* From the superposition principle, the potential generated by the interior charges is given by

$$V^<(\boldsymbol{r}') = \int_0^{r_{\text{cut}}} \mathrm{d}^3\boldsymbol{r}\, \frac{\rho^<(\boldsymbol{r})}{\|\boldsymbol{r} - \boldsymbol{r}'\|^p}. \tag{S41}$$

Rewriting $1/\|\boldsymbol{r} - \boldsymbol{r}'\|^p$ using the generalized Laplace expansion (Eq. S29), we obtain

$$V^<(\boldsymbol{r}') = \int_0^{r_{\text{cut}}} \mathrm{d}^3\boldsymbol{r}\, \rho^<(\boldsymbol{r}) \sum_{nlm} \frac{4\pi}{2l+1} A^p_{n,l} \frac{r^{l+2n}}{r'^{p+l+2n}} Y_l^m(\boldsymbol{r}) Y_l^m(\boldsymbol{r}') \tag{S42}$$

If $\rho^<$ is continuous, it is permissible to interchange the summation with the integral, which leads to

$$V^<(\boldsymbol{r}') = \sum_{nlm} \underbrace{\left[ \frac{4\pi A^p_{n,l}}{2l+1} \int_0^{r_{\text{cut}}} \mathrm{d}^3\boldsymbol{r}\, \rho^<(\boldsymbol{r}) r^{l+2n} Y_l^m(\boldsymbol{r}) \right]}_{=:M^<_{nlm}} \frac{1}{r'^{p+l+2n}} Y_l^m(\boldsymbol{r}') = \sum_{nlm} M^<_{nlm} \frac{1}{r'^{p+l+2n}} Y_l^m(\boldsymbol{r}') \tag{S43}$$

with

$$M^<_{nlm} = \frac{4\pi A^p_{n,l}}{2l+1} \int_0^{r_{\text{cut}}} \mathrm{d}^3\boldsymbol{r}\, \rho^<(\boldsymbol{r}) r^{l+2n} Y_l^m(\boldsymbol{r}). \tag{S44}$$

Thus, using the identical steps as for the Coulombic case, we obtain the desired result. □

### 3. Exterior Charges

Just as for the Coulomb potential, we can now flip the roles between the exterior and interior regions: the charges are now outside, and we wish to compute the potential generated by these in the interior region. The result is analogous to the previous case, except that all factors of $r^{l+2n}$ and $1/r'^{p+l+2n}$ switch roles.

**Theorem S1.7.** *Let $\rho^>$ be a charge density which is entirely contained outside of a cutoff radius $r_{\text{cut}}$. The resulting "electrostatic" (inverse power-law) potential $V^>(\boldsymbol{r})$ with exponent $p$ evaluated at some point $\boldsymbol{r}$ inside of the cutoff is given by*

$$V^>(\boldsymbol{r}) = \sum_{nlm} M^>_{nlm} r^{l+2n} Y^m_l(\hat{\boldsymbol{r}}), \tag{S45}$$

*with coefficients*

$$M^>_{nlm} = \frac{4\pi}{2l+1} A^p_{n,l} \int_{r_{\text{cut}}}^{\infty} \mathrm{d}^3\boldsymbol{r}' \, \frac{1}{r'^{p+l+2n}} Y^m_l(\hat{\boldsymbol{r}}')\rho^<(\boldsymbol{r}'), \tag{S46}$$

*and where $\sum_{nlm}$ is a shorthand for $\sum_{n=0}^{\infty}\sum_{l=0}^{\infty}\sum_{m=-l}^{l}$.*

*Proof.* The proof is completely analogous to the various versions presented so far, consisting of the steps:

1. Start from the expression $V^>(\boldsymbol{r}) = \int_{r_{\text{cut}}}^{\infty} \mathrm{d}^3\boldsymbol{r}' \, \frac{\rho^>(\boldsymbol{r}')}{\|\boldsymbol{r}-\boldsymbol{r}'\|^p}$ (Eq. (S3))
2. Use the Laplace expansion (Eq. (S29)) for $1/\|\boldsymbol{r}-\boldsymbol{r}'\|^p$
3. Interchange the order of summation (over $n, l, m$) and integration
4. Regroup factors that depend on $\boldsymbol{r}'$ to get the coefficients $M^>_{nlm}$

□

### 4. Inter-Regional Interaction Energy

Finally, we discuss how to compute the "inter-regional" interaction energy $E_{\text{int}}$ between the charges in the two regions, namely

$$E_{\text{int}} = \int_0^{r_{\text{cut}}} \mathrm{d}^3\boldsymbol{r} \int_{r_{\text{cut}}}^{\infty} \mathrm{d}^3\boldsymbol{r}' \, \frac{\rho^<(\boldsymbol{r})\rho^>(\boldsymbol{r}')}{\|\boldsymbol{r}-\boldsymbol{r}'\|^p}. \tag{S47}$$

As for the Coulomb potential, obtaining a multipolar expression for this interaction energy will be useful to obtain a physical interpretation of ML models that are built on top of the LODE features.

**Theorem S1.8.** *The interaction energy $E_{\text{int}}$ between the interior charges $\rho^<$ and exterior charges $\rho^>$ for a general exponent $p \neq 1$ can be computed as*

$$E_{\text{int}} = \sum_{nlm} \frac{2l+1}{4\pi A^p_{n,l}} M^>_{nlm} M^<_{nlm}. \tag{S48}$$

*where $M^>_{nlm}$ and $M^<_{nlm}$ are the exterior and interior multipole moments defined in the two previous subsections S1 C 3 and S1 C 2, respectively.*

*Proof.* The proof is completely analogous to the various versions presented so far, consisting of the steps:

1. Start from the expression $E_{\text{int}} = \int_0^{r_{\text{cut}}} \mathrm{d}^3\boldsymbol{r} \int_{r_{\text{cut}}}^{\infty} \mathrm{d}^3\boldsymbol{r}' \, \frac{\rho^<(\boldsymbol{r})\rho^>(\boldsymbol{r}')}{\|\boldsymbol{r}-\boldsymbol{r}'\|^p}$ (Eq. (S4))
2. Use the Laplace expansion (Eq. (S29)) for $1/\|\boldsymbol{r}-\boldsymbol{r}'\|^p$
3. Interchange the order of summation (over $n, l, m$) and integration
4. Group all factors that depend on $\boldsymbol{r}'$ together to get the coefficients $M^>_{nlm}$, and those that depend on $\boldsymbol{r}$ together to get the coefficients $M^<_{nlm}$

□

### D. Remark On Conventions and Prefactors

The definitions of the various multipolar quantities in this work might differ from those found in some of the literature. We briefly summarize some conventions.

- We write all results using the real versions of the spherical harmonics, since these are more suitable for our applications in which all functions are real-valued. The actual software implementation also uses real spherical harmonics due to more efficient storage.

  All results do however also apply if we use complex spherical harmonics instead, since the transformation between the two is unitary, with a single modification. In most places, the spherical harmonics appear in pairs. One of the two spherical harmonics (which one does not matter) will then need to get replaced by the complex conjugate. For the Laplace expansion of the Coulomb potential, this is explicitly shown at the end of the proof of Lemma S5.

- We refer to the coefficients $M^{<}_{lm}$ (or $M^{<}_{nlm}$) that characterize **interior** charges as **interior** multipole moments. On the other hand, some works would call this the **exterior** multipole expansion, since we evaluate the potential at a point $\boldsymbol{r}'$ in the exterior region (and vice versa if the charges are outside). We decided to use this terminology because the focus in this work is on the atoms (charges), rather than where the potential is evaluated.

- Our definition of multipole moments, e.g. those in sections S1 B 2 and S1 B 3 contain the prefactors of $\frac{4\pi}{2l+1}$. It would, however, also be possible not to include this factor in the coefficient itself, and to keep it in the final summation. This clearly does not affect any of the conclusions. The current convention was chosen to maximize the mathematical analogies to the density based descriptors which are discussed in more detail in the next section within this SI.

## S2. PHYSICAL INTERPRETATION AND OPTIMIZATION OF LODE REPRESENTATION

### A. Overview of this section

In this section, we provide a complete and mostly self contained description of the mathematical theory behind the LODE descriptors that are used throughout the main text. We begin by reviewing a general mathematical framework for the construction of atomic descriptors that unifies LODE and many SR features (e.g. SOAP) that is described in [2]. We believe that the way we present the concepts here will help to better see the connection between the different representations as well as the multipole expansion discussed in the previous section in this SI.

### B. General Framework for Atomic Representations

We begin by providing a quick summary of a general framework to construct atomic representations, using the better-established SR descriptors as an example. We are given an atomic structure consisting of $N$ atoms (with or without periodic boundary conditions) indexed as $i = 1, 2, \ldots, N$, whose position vectors are denoted by $\boldsymbol{r}_i$ and chemical species by $a_i \in \{\mathrm{H}, \mathrm{He}, \mathrm{Li}, \ldots\}$.

We start by defining a density contribution function $g$, a popular choice being a Gaussian function

$$g(\boldsymbol{r}) \propto \exp(-\boldsymbol{r}^2/2\sigma^2), \tag{S49}$$

where $\sigma$ is a parameter controlling the width, as shown in Fig. S2 Ba. Different normalizations for the Gaussian are possible, but the specific choice is irrelevant to this discussion.

This density contribution function $g$ is then used to define a density function $\rho$ over the entire structure, $\rho(\boldsymbol{r}) = \sum_j g(\boldsymbol{r} - \boldsymbol{r}_j)$ shown in Fig. S2 Bb. This function $\rho$ is not directly related to any physical quantity (e.g. the electron density), but contains the information about the location of all atoms in the structure. For instance, we could imagine that we "hide" all atoms from Fig. S2 Bb, and only show the density function. Since the locations of the atoms correspond to peaks in $\rho$, we can reconstruct the atomic positions (up to some precision that is determined by the smearing $\sigma$).

To describe the local neighborhood around an atom $i$ rather than the entire structure, we use the atom centered density $\rho_i(\boldsymbol{r}) = \rho(\boldsymbol{r} + \boldsymbol{r}_i)$, truncated at some cutoff radius $r = \|\boldsymbol{r}\| \leq r_{\mathrm{cut}}$, i.e. only the portion of $\rho$ around $\boldsymbol{r}_i$ (the cutoff is shown with dashed lines in Fig. S2 Bc).

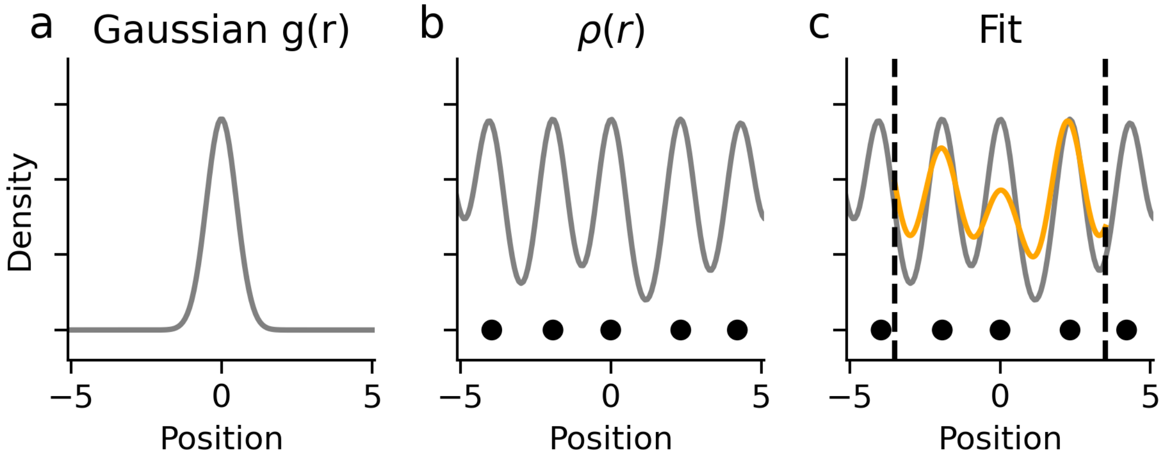


Figure S4. Visualization of the steps involved to generate short-range descriptors, including the popular SOAP descriptor. a: Density contribution function showing the density for a single atom. b: Density of the structure as a whole, obtained by considering superpositions of the function in part a for each atom. c: Fitting the target density within some cutoff requires the specification of some fitting parameters, which contain the information on the atomic positions.

For computational applications, it is necessary to describe the neighborhood of atom $i$ using a discrete set of coefficients, rather than an abstract function $\rho_i$. Thus, we choose a set of orthonormal basis functions $B_{nlm}$, which for symmetry reasons are typically of the form $B_{nlm}(\boldsymbol{r}) = R_{nl}(r)Y_l^m(\hat{\boldsymbol{r}})$, where $R_{nl}(r)$ are the radial basis functions and $Y_l^m(\hat{\boldsymbol{r}})$ are the real spherical harmonics describing the angular part. Any continuous function including $\rho_i$ can then be written as the linear combination of the basis functions

$$\rho_i(\boldsymbol{r}) = \sum_{nlm} \rho_{i,nlm} B_{nlm}(\boldsymbol{r}) = \sum_{nlm} \rho_{i,nlm} R_{nl}(r) Y_l^m(\hat{\boldsymbol{r}}), \tag{S50}$$

with coefficients $\rho_{i,nlm}$ given by the inner product of the basis function with the target density $\rho_i$,

$$\rho_{i,nlm} = \int_0^{r_{\text{cut}}} \mathrm{d}^3\boldsymbol{r}\, R_{nl}(r) Y_l^m(\hat{\boldsymbol{r}}) \rho_i(\boldsymbol{r}). \tag{S51}$$

The coefficients $\rho_{i,nlm}$ contain the information about the atomic positions around atom $i$, and can thus be used in ML applications to predict atomic properties. In reality, in most applications, the coefficients are not used directly: for instance, if the target property is invariant under rotations (e.g. the energy), rotationally invariant combinations of these coefficients are used. This can also be generalized to arbitrary transformation behaviors with respect to rotations.

The SR nature of the descriptor arises from the use of a quickly decaying function for the density contribution function $g$, common choices being the aforementioned Gaussian function [3, 4] and the infinitely sharp limit of delta distributions $g(\boldsymbol{r}) \to \delta(\boldsymbol{r})$ [5, 6], which in turn enables efficient predictions of materials properties scaling linearly with the number of atoms. More details on SR descriptors are discussed in the review article [2].

### C. LODE for Coulombic Interactions

While this framework was originally developed for SR descriptors, it permits an elegant extension to arbitrary LR interactions. By changing the density contributions $g$ to a slowly decaying function, we obtain a new density function $\rho(\boldsymbol{r})$ for which even the local neighborhood around an atom $i$ contains more information about far-away atoms.

Motivated by the fact that the most important LR interaction is the electrostatic one, the original work on LODE [7] used a density contribution of the form

$$g_{\text{Coulomb}}(\boldsymbol{r}) = \frac{\operatorname{erf}\left(r/\sqrt{2}\sigma\right)}{r}, \tag{S52}$$

where $\operatorname{erf}(x)$ is the error function. This corresponds to the Coulomb potential of a Gaussian charge density, commonly used for Ewald summation [1]. As for the Coulomb potential, this function asymptotically behaves as $1/r$ for $r \to \infty$,

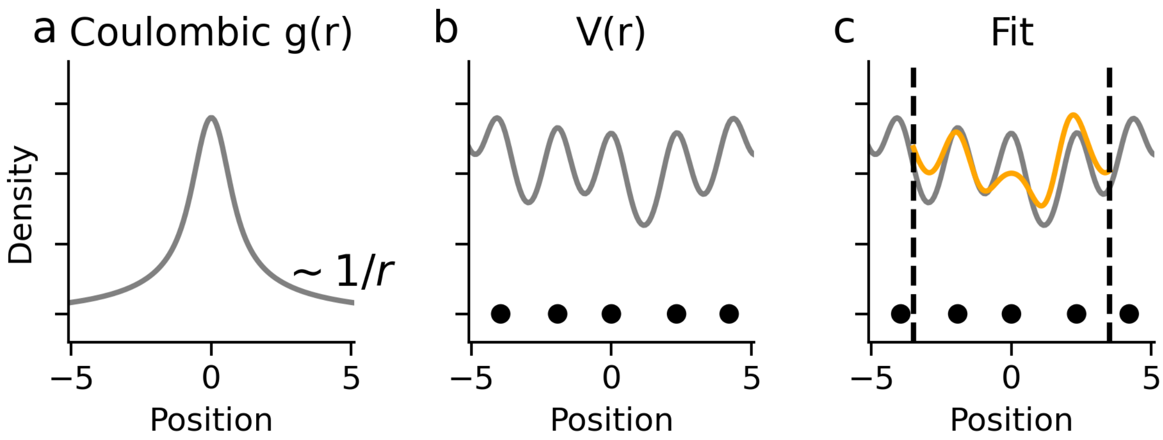


Figure S5. Visualization of the steps involved to generate the LODE descriptors. a: Density contribution function showing the density for a single atom. As opposed to a Gaussian, the functions now decay as $1/r$. b: Density of the structure as a whole, obtained by considering superpositions of the function in part a for each atom. c: Fitting the target density within some cutoff requires the specification of some fitting parameters, which contain the information on the atomic positions, now also including atoms outside of the cutoff due to the slow decay.

while the singularity at $r = 0$ of the bare Coulomb potential has been smeared out (Fig. S2 Ca). To differentiate this Coulombic density from the SR ones, as well as to emphasize the mathematical analogy to the Coulomb potential of the structure, we write $V(\boldsymbol{r}) = \sum_j g_{\text{Coulomb}}(\boldsymbol{r}-\boldsymbol{r}_j)$ rather than $\rho(\boldsymbol{r})$ for the total density which is shown in Fig. S2 Cb.

Just as for SR densities, for each center atom $i$, an atomic descriptor is constructed by first defining the shifted (atom centered) version of the density, $V_i(\boldsymbol{r}) = V(\boldsymbol{r} - \boldsymbol{r}_i)$ defined up to $r = \|\boldsymbol{r}\| \leq r_{\text{cut}}$. To get a discrete set of coefficients, this density is projected onto the basis functions $B_{nlm}$, leading to coefficients

$$V_{i,nlm} = \int_0^{r_{\text{cut}}} \mathrm{d}^3\boldsymbol{r}\, R_{nl}(r) Y_l^m(\hat{\boldsymbol{r}}) V_i(\boldsymbol{r}). \tag{S53}$$

The key idea is that due to the slow decay, even atoms outside the cutoff will provide significant contributions to the interior density (Fig. S2 Cc). The only conceptual difference to the SR version is thus a different choice of the density contribution $g(\boldsymbol{r})$, which allows us to easily reuse all ML methods that work for SR models and combine them with the LR modifictions. This is the key idea of the LODE framework.

Note that for systems with periodic boundary conditions, the sum $V(\boldsymbol{r}) = \sum_j g(\boldsymbol{r} - \boldsymbol{r}_j)$ is understood to include all periodic images. While only the nearest ones are sufficient for SR models due to the (at least exponentially) fast decay of $g(r)$, the LR descriptors require a more proper treatment of the infinitely many periodic images using an Ewald-like Fourier space formulation, which is discussed in Section S3. Thus, while conceptually close to SR densities, actual implementations to compute the coefficients $V_{i,nlm}$ will be quite different from their SR counterparts.

### D. Extension to Arbitrary Long-Range Descriptors

Given the diversity of $1/r^p$ interactions, $1/r^6$ being the most important from a physical point of view, it is natural to extend LODE to other exponents $p$. This can be achieved by finding a function $g(\boldsymbol{r})$ behaving as $1/r^p$ for $r \to \infty$, while being monotonous in $r$ and differentiable in the entire space. We use

$$g_p(\boldsymbol{r}) = \frac{1}{\Gamma\left(\frac{p}{2}\right)} \frac{\gamma\left(\frac{p}{2}, \frac{r^2}{2\sigma^2}\right)}{r^p}, \tag{S54}$$

where $\Gamma(x)$ is the Gamma function, and $\gamma(a, x)$ is the lower incomplete Gamma function. Up to different scaling, this is a functional form that was first introduced in [8] and extended in [9, 10].

It should be noted that (S54) is not simply the effective $1/r^p$ potential generated by a Gaussian charge density, which would naively be the first candidate function. In fact, such an approach would not work for exponents $p \geq 3$ due to the strong singularity at the origin. Nevertheless, (S54) reduces to eq. (S52) for $p = 1$. Some mathematical

details of this density contribution function, including the fact that it satisfies all desired properties, are discussed in section S4.

Summarizing the general recipe to generate the descriptors discussed so far, the methods are defined by the choices of (1) the density contributions $g(\boldsymbol{r})$ and (2) the radial basis functions $R_{nl}(r)$ on which the resulting density is projected. Different SR models as well as the transition to various LR models is primarily characterized by the choice of $g(\boldsymbol{r})$. In the next two subsections, we show how a suitable choice of $R_{nl}$ leads to a clean physical interpretation of descriptors as well as more efficient implementations. While all $1/r^p$ potentials share many properties with the Coulombic special case of $p = 1$, the general case is more complicated and is discussed separately after building a good intuition based on the Coulomb potential first.

### E. Physical Interpretation and Optimizations for the Coulombic Case

So far, we have provided a mathematical recipe to compute both SR and LODE features, including the generalization to arbitrary exponents $p$. We will now show how a more detailed mathematical analysis can provide both a more physical interpretation of these coefficients, as well as a mathematical optimization method for more efficient implementations.

In terms of mathematical prerequisites, the rest of this section will make use of two key properties of spherical harmonics. The first one is the mutual orthogonality, explicitly given by

$$\int_{S^2} \mathrm{d}S\, Y_l^m(\hat{\boldsymbol{r}}) Y_{l'}^{m'}(\hat{\boldsymbol{r}}) = \int_0^{2\pi} \mathrm{d}\phi \int_0^{\pi} \mathrm{d}\theta\, \sin\theta Y_l^m(\theta,\phi) Y_{l'}^{m'}(\theta,\phi) = \delta_{l,l'}\delta_{m,m'}, \tag{S55}$$

where $S^2$ is the unit sphere characterized by the two spherical angles $\theta$ and $\phi$. The second property is that any continuous (more generally, $L^2$) function $f$ in the angles $(\theta, \phi)$ (on the sphere $S^2$) can be expressed as a Fourier series

$$f = \sum_{l,m} f_{l,m} Y_l^m, \tag{S56}$$

with coefficients

$$f_{l,m} = \int_{S^2} \mathrm{d}S\, Y_l^m f. \tag{S57}$$

Summarizing the two properties more compactly, we can say that the spherical harmonics form an orthonormal (Schauder) basis for the ($L^2$)-space of functions on the unit sphere.

The last key ingredient for our analysis is the multipole expansion from electrostatics, which was already used in [11]. That work in fact claimed that

> ... neither the atom density $\rho_i$ nor the associated potential $V_i$ correspond to physical quantities ...

and that only certain combinations of $\rho_{i,nlm}$ and $V_{i,nlm}$

> ... entail(s) formal similarities with physics-based electrostatic models.

We will show that a more careful analysis using the multipole expansion does in fact provide a direct physical interpretation to both sets of coefficients $\rho_{i,nlm}$ and $V_{i,nlm}$ in terms of electrostatic quantities. This connection also provides us with an explicit recipe for faster algorithmic implementations. A self contained review of the multipole expansion for the Coulomb potential, as well as an extension to arbitrary exponents $p$ that was performed as part of this work, are discussed in section S1 C. For readers only interested to the applications to atomistic descriptors, we briefly summarize the main results.

Let $\rho_i$ be the atomic density around atom $i$, but now without the restriction due to a cutoff radius. As shown in Fig. S1a, we split it up into an interior part $\rho_i^<$ and exterior part $\rho_i^>$, each only containing the density inside / outside the cutoff radius $r_{\mathrm{cut}}$, respectively, such that $\rho_i = \rho_i^< + \rho_i^>$. For the rest of this document, we shall denote by $\boldsymbol{r}$ ($\boldsymbol{r}'$) a point inside (outside) the cutoff, i.e. $r = \|\boldsymbol{r}\| < r_{\mathrm{cut}}$ ($r' = \|\boldsymbol{r}'\| > r_{\mathrm{cut}}$).

The classical version of the multipole expansion is discussed in many textbooks on electrodynamics [1], and is illustrated in Fig. S1b: The electric potential $V_i^<(\boldsymbol{r}')$ generated by a localized (interior) charge density $\rho_i^<$ evaluated at some point $\boldsymbol{r}'$ in the exterior region can be written as

$$V_i^<(\boldsymbol{r}') = \sum_{lm} M_{i,lm}^< \frac{1}{r'^{l+1}} Y_l^m(\hat{\boldsymbol{r}}'), \tag{S58}$$

with coefficients

$$M_{i,lm}^{<} = \int_0^{r_{\text{cut}}} \mathrm{d}^3\boldsymbol{r}\, r^l Y_l^m(\hat{\boldsymbol{r}}) \rho_i^{<}(\boldsymbol{r}), \tag{S59}$$

which are called (interior) multipole moments and completely characterize the potential in the exterior region. Intuitively, this corresponds to a Fourier-like expansion of the interior density into terms of higher and higher frequencies.

Comparing this with (S51), we can see that the SR features $\rho_{i,nlm}$ can be made to exactly match the interior multipole moment $M_{i,lm}^{<}$ of the density $\rho_i^{<}$ within the cutoff radius around atom $i$, if we choose the radial basis function $R_{nl}(r) = r^l$, which provides us with SR features that have an exact electrostatic interpretation.

Flipping the roles around, it is possible to compute the elctrostatic potential $V_i^{>}(\boldsymbol{r})$ generated by the exterior charges $\rho_i^{>}$, evaluated at an interior point $\boldsymbol{r}$, as is shown in Fig. S1c. Similar to the previous case, the potential is completely characterized by coefficients $M_{i,lm}^{>}$, the exterior multipole moments, such that

$$V_i^{>}(\boldsymbol{r}) = \sum_{lm} M_{i,lm}^{>} r^l Y_l^m(\hat{\boldsymbol{r}}), \tag{S60}$$

$$M_{i,lm}^{>} = \int_{r_{\text{cut}}}^{\infty} \mathrm{d}^3\boldsymbol{r}'\, \frac{1}{r'^{l+1}} Y_l^m(\hat{\boldsymbol{r}}') \rho_i^{>}(\boldsymbol{r}'). \tag{S61}$$

As for the interior version, this can be interpreted as a decomposition of the exterior charge density $\rho^{>}$ into (angular) frequency components.

To show the analogy to the LODE coefficients, we now project this density $V_i^{>}(\boldsymbol{r})$ onto basis functions $B_{nlm}(\boldsymbol{r}) = R_{nl}(r) Y_l^m(\hat{\boldsymbol{r}})$. From the orthonormality of the spherical harmonics, we get

$$V_{i,nlm}^{>} = \int_0^{r_{\text{cut}}} \mathrm{d}^3\boldsymbol{r}\, R_{nl}(r) Y_l^m(\hat{\boldsymbol{r}}) V_i^{>}(\boldsymbol{r}) = M_{i,lm}^{>} \int_0^{r_{\text{cut}}} \mathrm{d}r\, r^{2+l} R_{nl}(r) \tag{S62}$$

Thus, we can see that the projection of $V_i^{>}$ allows us to recover the exterior multipole moment $M_{i,lm}^{>}$ up to a prefactor that only depends on the choice of radial basis. Choosing the same radial function $R_{nl}(r) = R_l(r) = r^l$, we obtain

$$V_{i,lm} = C_l M_{i,lm}^{>}, \quad C_l = \frac{r_{\text{cut}}^{3+2l}}{3+2l}. \tag{S63}$$

Thus, if it was possible to extract from the full potential $V_i(\boldsymbol{r})$ the part $V_i^{>}(\boldsymbol{r})$ that corresponds to the contribution of exterior charges, a comparison with eq. (S53) shows that the LODE coefficients $V_{i,nlm}$ correspond precisely to the exterior multipole moment $M_{i,lm}^{>}$, for the charge density $\rho_i^{>}$ defined relative to the central atom $i$. Eliminating the interior part $\rho_i^{<}$ is simple in principle, since this can be implemented using the same methods as for SR densities.

There are two important messages that we can learn from this analysis. Firstly, beyond the formal analogy originally proposed in [11] for the special case of linear models, we can see that the coefficients $\rho_{i,nlm}$ and a suitable modification of $V_{i,nlm}$ correspond exactly to the interior and exterior multipole moments of the "density" $\rho_i(\boldsymbol{r})$ centered around atom $i$, if we interpret it as a charge density (see remarks in section S3 of the SI regarding the sign conventions and the more subtle treatment of different chemical species) separated into two regions by the cutoff radius $r_{\text{cut}}$ around center atom $i$.

Secondly, we can connect this to a significant speedup of codes implementing LODE. While typical approaches for ML models use a large number of radial basis functions, $n = 1, 2, \ldots, n_{\max}$ on the order of $4 \sim 10$, this analysis shows us that the entire LR information about atoms outside of the cutoff can be captured by using a single radial basis function, namely $r^l$. This results in a reduction of the computational cost as well as memory of LODE by a factor of $n_{\max}$, which can be close to an order of magnitude.

### F. Physical Interpretation and Optimizations for General Exponents

We now extend this analysis to exponents other than $p = 1$. Firstly, we need to start by deriving a generalization of the multipole expansion that is suitable for our use case. While different such forms have been proposed, either based on the use of Cartesian coordinates or modified spherical harmonics, these methods are less suitable for many ML applications, that require a more systematic expansion in terms of the (usual) spherical harmonics.

Stating the main result first, we will show that the potential $V_i^{>}(\boldsymbol{r})$ at a point $\boldsymbol{r}$ in the interior region generated by an exterior charge density $\rho_i^{>}(\boldsymbol{r}')$ can be written as

$$V_i(\boldsymbol{r}) = \int_{r_{\text{cut}}}^{\infty} \mathrm{d}^3\boldsymbol{r}''\, \frac{\rho_i(\boldsymbol{r}')}{\|\boldsymbol{r} - \boldsymbol{r}'\|^p} = \sum_{nlm} M_{i,nlm}^{>} r^{l+2n} Y_l^m(\hat{\boldsymbol{r}}), \tag{S64}$$

where $M^{>}_{i,nlm}$ are suitable generalizations of the multipole moments that completely characterize the potential within the cutoff sphere. Similarly to the Coulombic special case, we can extract these coefficients and use them as inputs to a ML model using a suitable radial basis.

This form shows one key difference: The sum now also runs over $n = 0, 1, 2$, etc., indicating a more complicated radial dependence. The underlying mathematical reason is the fact that the Coulomb potential $g(\boldsymbol{r}) = 1/r$ is a solution to the Laplace equation $\Delta g = 0$ for $\boldsymbol{r} \neq 0$, while this is no longer true for any other $p \neq 1$.

Just as for the Coulombic case, we can extract the coefficients $M^{>}_{i,nlm}$ by choosing an appropriate set of radial basis functions $R_{nl}(r)$, the extra complication being the fact that for each angular channel $l$, the radial dependence is no longer a simple function with a single coefficient.

Nevertheless, keeping in mind that the term with $M^{>}_{i,nlm}$ in the generalized multipole expansion discussed in section S1 C 3 contains information about the density decaying as $1/r^{p+l+2n}$, we propose the following method to pick the best exponents. First, one chooses a maximal decay exponent $1/r^{p_{\max}}$, with $p_{\max} = p + l_{\max}$. Then, we use all coefficients $M^{>}_{i,nlm}$ for which $p + l + 2n < p_{\max}$ as input to our ML model. This allows us to interpret the cutoff as a truncation in decay speed of the potentials. For a given level of desired accuracy $p_{\max}$, this approach requires about half as many coefficients compared to a more naive implementation in which a range of values for $l$ and $n$ are specified independently.

### G. Building ML Models

A connection between LODE and the multipole expansion was already mentioned in previous work [11] for the special case of linear models, the key difference being that (1) beyond being a mathematical analogy, we see that the LODE coefficients are *precisely* suitably defined multipole moments characterizing the interior and exterior atoms, and (2) the mathematical equivalence arises directly at the level of the coefficients, and is not restricted to the use of linear models.

While our discussion so far has focused entirely on the descriptors, and not on the model, it is important to discuss the final step that will lead to the actual target property.

Just as for SR descriptors, we know that the power spectrum coefficients of the form

$$\sum_{m=-l}^{l} \rho_{i,nlm} V_{i,n'lm} \tag{S65}$$

for any $n, n', l$ are rotationally invariant, and can thus be used as inputs to predict invariant target properties like the energy or charge of a system. While many other invariants can be constructed in a similar manner, these specific ones allow for a particularly simple interpretation.

To find an analogous quantity in electrostatics, let $\rho$ once again be an arbitrary charge density, divided up into an interior and exterior part relative to some origin. The electrostatic interaction energy $E_{\text{int}}$ between the interior charges $\rho^{<}$ and exterior charges $\rho^{>}$ (but not the interactions among themselves) is then given by

$$E_{\text{int}} = \int_0^{r_{\text{cut}}} \mathrm{d}^3\boldsymbol{r} \int_{r_{\text{cut}}}^{\infty} \mathrm{d}^3\boldsymbol{r}' \, \frac{\rho^{<}(\boldsymbol{r})\rho^{>}(\boldsymbol{r}')}{\|\boldsymbol{r} - \boldsymbol{r}'\|}. \tag{S66}$$

Using the multipole expansion, it can be shown that

$$E_{\text{int}} = \sum_{lm} \frac{2l+1}{4\pi} M^{>}_{lm} M^{<}_{lm}. \tag{S67}$$

In other words, the interaction energy is completely specified by knowing both the interior and exterior multipole moments of the charge distribution.

Beyond the Coulomb potential, the proof of the general multipole expansion for arbitrary exponents $p$ can be used to also obtain the analogous result

$$E_{\text{int}} = \int_0^{r_{\text{cut}}} \mathrm{d}^3\boldsymbol{r} \int_{r_{\text{cut}}}^{\infty} \mathrm{d}^3\boldsymbol{r}'\,' \frac{\rho^{<}(\boldsymbol{r})\rho^{>}(\boldsymbol{r}')}{\|\boldsymbol{r} - \boldsymbol{r}'\|^p} = \sum_{nlm} \frac{2l+1}{4\pi A^p_{l,n}} M^{<}_{nlm} M^{>}_{nlm}. \tag{S68}$$

This can be compared with a linear model on the invariants in Eq. S65 to predict the "atomic energy" $E_i$,

$$E_i = \sum_{nn'lm} E_{nn'l} \rho_{i,nlm} V_{i,n'lm}. \tag{S69}$$

Remembering that $\rho_{i,nlm}$ can be chosen to essentially correspond to $M^{<}_{nlm}$, while $V_{i,nlm}$ is $M^{>}_{nlm}$ for the charge density centered around atom $i$, we can see that we essentially recover the same mathematical form as the actual interaction energy between the two regions discussed in section S1, with the extra flexibility of choosing the coefficients $E_{nn'l}$ in a non-uniform way. This is essentially the result presented in [11] rewritten in our notation, but with a cleaner separation of the connection between the multipole moments and the final model.

Clearly, the usage of the LODE coefficients $V_{i,nlm}$ is not restricted to linear models, and thanks to the mathematical closeness to SR approaches, any software architecture that works with SR descriptors should be capable of seemlessly integrating LODE to incorporate far-field contributions. Furthermore, the coefficients $V_{i,nlm}$ also posses the full equivariance discussed in [12], and can thus be used to learn target properties of arbitrary tensorial character including dipole moments or electron densities.

## S3. SIMILARITIES AND DIFFERENCES OF THE LODE DENSITY WITH THE ACTUAL COULOMB POTENTIAL

The density function $V(\boldsymbol{r})$ that is used throughout the LODE framework is, by construction, closely related to the Coulomb potential. This is also why, to help the intuition, we informally refer to it as "the potential (field)" throughout this document. There are, however, two subtle differences to the actual Coulomb potential that one might compute, e.g. for MD simulations.

Summarized in a few sentences each, these are:

- Traditional methods for electrostatics including the Ewald based ones or PPPM split the potential into a SR and LR part, and treats the LR part with Fourier transforms for efficient evaluation. In this picture, LODE basically only is using the LR part.
- In MD, each atom is assigned a charge $q_i$ (often one charge per chemical species), and the potential is the sum of the bare $1/r$ potential weighted by the charges. In LODE, each chemical species is assigned a separate density field, and are thus treated completely independently.

In the following two subsections, each of these points is discussed further.

### A. Absence of SR-LR splitting

For the Coulombic case, it is possible to interpret the resulting function $g_{\mathrm{Coulom}}(r)$ as the effective potential generated by a Gaussian charge density, which is also how Ewald summation if often motivated in textbooks. This way of introducing the function $g(r)$ certainly has the advantage of being visually and physically pleasing, since the resulting method has a clear interpretation. In such a case, the total Coulomb potential is split into a SR and LR part, namely

$$\frac{1}{r} = g(r) + h(r) = \frac{\mathrm{erf}(r/\sqrt{2}\sigma)}{r} + \frac{\mathrm{erfc}(r/\sqrt{2}\sigma)}{r}, \tag{S70}$$

where the second term $h(r)$ is the SR part containing the complementary error function $\mathrm{erfc}(x) = 1 - \mathrm{erf}(x)$.

Splitting the Coulomb potential in this way has the advantage that the first term is purely LR, and thus easy to calculate in practice using Fourier transforms, while the second term is SR, and can thus be efficiently evaluated in real space. In traditional molecular dynamics simulations, explicitly including the SR part is important to get accurate energy and force predictions. LODE, on the other hand, only includes the LR part of this decomposition, the idea being that the SR part is typically already well covered by established approaches.

### B. Treatment of different chemical species

A second way in which the LODE density function $V(\boldsymbol{r})$ differs from the usual electrostatic potential is the treatment of different atomic species. At the simplest level, in traditional MD simulations, each atomic species is assigned a charge $q$ (e.g. for NaCl, one could set $q_{\mathrm{Na}} = +1$ and $q_{\mathrm{Cl}} = -1$ in appropriate units). The "physical" electrostatic potential $V_{\mathrm{Coulomb}}(\boldsymbol{r})$ then formally corresponds to the expression

$$V_{\mathrm{Coulomb}}(\boldsymbol{r}) = \sum_j q_j g_{\mathrm{bare}}(\|\boldsymbol{r} - \boldsymbol{r}_j\|), \tag{S71}$$

where the sum runs over all atoms in the structure (in general, including periodic images), and $g_{\mathrm{bare}}(r) = 1/r$ is the (bare) Coulomb potential. In other words, regardless of the number of chemical species present in the system, we only obtain one potential function $V_{\mathrm{Coulomb}}(\boldsymbol{r})$.

For LODE, on the other hand, each species is treated separately. Taking NaCl as an example, we would then obtain two separate density functions, namely

$$V_{\mathrm{Na}}(\boldsymbol{r}) = \sum_{j \in \mathrm{Na}} g(\|\boldsymbol{r} - \boldsymbol{r}_j\|) \tag{S72}$$

$$V_{\mathrm{Cl}}(\boldsymbol{r}) = \sum_{j \in \mathrm{Cl}} g(\|\boldsymbol{r} - \boldsymbol{r}_j\|), \tag{S73}$$

where the sum in the first (second) line only runs over all Na (Cl) atoms, respectively, including their periodic images. Note also that the charges $q_j$ in the summation has been removed. Furthermore, the bare potential $g_{\mathrm{bare}}(r) = 1/r$ has been replaced by the appropriate smeared version $g(r)$. We shall not touch upon this point since it was already discussed in the previous subsection. These two functions could be called the "Na-potential" and "Cl-potential", respectively. The "physical" Coulomb potential, if we ignore the distinction between $g_{\mathrm{bare}}$ and $g$, then is simply the linear combination

$$V_{\mathrm{Coulomb}}(\boldsymbol{r}) = q_{\mathrm{Na}} V_{\mathrm{Na}}(\boldsymbol{r}) + q_{\mathrm{Cl}} V_{\mathrm{Cl}}(\boldsymbol{r}). \tag{S74}$$

From the point of view of ML models, it means that the information about the "physical" Coulomb potential is contained in the LODE potentials, but the latter still have more flexibility, and describe the location of the atoms separately for each species.

Clearly, in a data set containing atoms of $N_a$ different species, there would be one such potential $V_a$ for each species, where $a$ runs over all possible such elements.

All the steps discussed in the main text are then separately applied to each of these potentials. Thus, after picking a center atom $i$ for which we wish to compute the atom-centered features, we compute the potential function for species $a$ centered around atom $i$, as $V_{ia}(\boldsymbol{r}) = V_a(\boldsymbol{r} - \boldsymbol{r}_i)$ and project onto a basis, leading to a set of coefficients $V_{ia,nlm}$ defined by

$$V_{ia} = \sum_{nlm} V_{ia,nlm} B_{nlm}. \tag{S75}$$

One further subtlety has to be considered for periodic systems: for the traditional Ewald summation based methods, it can be shown that (for exponents $p < 3$, which includes the important Coulomb case) the well-definedness of the potential function requires that the unit cell as a whole is charge neutral. This condition is relatively easy to satisfy for systems, in which the charges $q_j$ are chosen manually. On the other hand, as is apparent from equations (S72) and (S73), all terms in the summation are assigned the same charge. Physically, this problem can be solved by adding a homogeneous background charge of opposite sign to the system, as is also done for, e.g. the Jellium model.

## S4. BEHAVIOR OF GENERAL DENSITY CONTRIBUTION FUNCTION

We show that the density contribution function

$$g(\boldsymbol{r}) = g(r) = \frac{1}{\Gamma\left(\frac{p}{2}\right)} \frac{\gamma\left(\frac{p}{2}, \frac{r^2}{2\sigma^2}\right)}{r^p}, \tag{S76}$$

has the desired mathematical properties, namely that it behaves as $1/r^p$ as $r \to \infty$ while removing the singularity at the origin.

The Gamma function is defined as

$$\Gamma(a) = \int_0^\infty t^{a-1} e^{-t} \mathrm{d}t, \tag{S77}$$

while the lower incomplete Gamma function is defined similarly, but the integration range restricted to $[0, x]$:

$$\gamma(a, x) = \int_0^x t^{a-1} e^{-t} \mathrm{d}t. \tag{S78}$$

### A. Long-Range Limit

In the limit as $r \to \infty$, we want $g(r)$ to asymptotically behave as $1/r^p$. From the definition of the lower incomplete Gamma function, we can immediately obtain

$$\gamma(a,x) = \int_0^x t^{a-1} e^{-t} \mathrm{d}t \overset{x\to\infty}{\longrightarrow} \int_0^\infty t^{a-1} e^{-t} \mathrm{d}t = \Gamma(a) \tag{S79}$$

Thus, we can indeed see that

$$g(r) \sim \frac{1}{r^p} \quad \text{as} \quad r \to \infty, \tag{S80}$$

where the equivalence relation $f(x) \sim g(x)$ for $x \to x_0$ means that $f$ and $g$ asymptotically behave in the same way, formally defined as $\lim_{x\to x_0} \frac{f(x)}{g(x)} = 1$.

### B. Short-Range Limit

To convince ourselves that the singularity at $r = 0$ is properly taken care of, we can use the asymptotic expansion

$$\gamma(a,x) = \frac{x^a}{a} + O(x^{a+1}) \tag{S81}$$

as $x \to 0$, which can directly be obtained from Taylor expanding the exponential function, and using Fubini's theorem to interchange the order of summation and integration (since the integrand is absolutely integrable):

$$\gamma(a,x) = \int_0^x t^{a-1} \sum_{n=0}^\infty (-1)^n \frac{t^n}{n!} \mathrm{d}t = \sum_{n=0}^\infty \frac{(-1)^n}{n!} \int_0^x t^{a-1} t^n \mathrm{d}t = \sum_{n=0}^\infty \frac{(-1)^n}{n!} \frac{x^{a+n}}{a+n} \tag{S82}$$

$$= \frac{1}{a} x^a + O(x^{a+1}). \tag{S83}$$

Using this, we can see that the limit at $r \to 0$ is indeed a well defined nonzero value, namely

$$\lim_{r\to 0} g(r) = \lim_{r\to 0} \frac{1}{\Gamma\left(\frac{p}{2}\right)} \frac{\gamma\left(\frac{p}{2}, \frac{r^2}{2\sigma^2}\right)}{r^p} = \lim_{r\to 0} \frac{1}{\Gamma\left(\frac{p}{2}\right)} \cdot \frac{1}{\frac{p}{2}} \left(\frac{r^2}{2\sigma^2}\right)^{\frac{p}{2}} \cdot \frac{1}{r^p} = \frac{1}{\Gamma(\frac{p+2}{2})\,(2\sigma^2)^{\frac{p}{2}}}. \tag{S84}$$

with corrections that are quadratic in $r$ for small nonzero $r > 0$.

### C. Coulombic Special Case

We begin by showing that for the special case of $p = 1$, we recover the Coulomb potential of a Gaussian density

$$g_{\mathrm{Coulomb}}(r) = \frac{\mathrm{erf}(r/\sqrt{2}\sigma)}{r}. \tag{S85}$$

Comparing with the general expression, it suffices to show that

$$\mathrm{erf}(r/\sqrt{2}\sigma) = \frac{\gamma\left(\frac{1}{2}, \frac{r^2}{2\sigma^2}\right)}{\Gamma(1/2)} = \frac{\gamma\left(\frac{1}{2}, \frac{r^2}{2\sigma^2}\right)}{\sqrt{\pi}} \tag{S86}$$

since the factor of $1/r$ is common to both. This equality follows directly from the definition of the error function

$$\mathrm{erf} z = \frac{2}{\sqrt{\pi}} \int_0^z e^{-t^2} \mathrm{d}t \overset{u=t^2}{=} \frac{1}{\sqrt{\pi}} \int_0^{z^2} u^{-\frac{1}{2}} e^{-u} \mathrm{d}u = \frac{\gamma\left(\frac{1}{2}, z^2\right)}{\sqrt{\pi}}. \tag{S87}$$

Plugging in $z^2 = \frac{r^2}{2\sigma^2}$, we obtain the desired result.

### D. Why Gaussian Densities cannot be used in the general case

As was shown in this section, the density contribution functions $g(r)$ have a well-defined limit as $r \to 0$. Naively, just as for the Coulombic special case, one could hope to achieve this by using the effective potential generated by a Gaussian charge density. This, however, would not work for $p \geq 3$.

The qualitative way of seeing this is to work in spherical coordinates and study the asymptotic scaling of the potential as $r \to 0$. While the bare $1/r$ potential has a singularity at the origin, the Coulomb potential generated by a Gaussian charge (or any continuous charge density for that matter) is still finite at the origin due to the extra factor of $r^2$ arising from the Jacobian in spherical coordinates. More generally, $1/r^p \cdot r^2 = r^{2-p}$ can be integrated without leading to singularities as long as $p < 3$. Thus, if we wish to have a set of densities $g_p(r)$ that also varies smoothly with respect to $p$, it is impossible to use Gaussian densities.

Instead, if we consider the effective $1/r^p$ potential generated by a spherically symmetric density $\rho(\boldsymbol{r})$, the potential at a point $\boldsymbol{r}$ is then given by

$$\phi(\boldsymbol{r}) = \int_{\mathbb{R}^3} \frac{\rho(\boldsymbol{r}')}{\|\boldsymbol{r} - \boldsymbol{r}'\|^p} = \frac{2\pi}{(2-p)r} \int_0^\infty \mathrm{d}r' r' \rho(r') \left[|r - r'|^{-p+2} - (r + r')^{-p+2}\right] \tag{S88}$$

In our case, $\phi(\boldsymbol{r})$ would correspond to the density contribution function $g(\boldsymbol{r})$. Using the specific form in Eq. (S76), one can invert the relation and compute what the effective charge density (or smearing) $\rho(r)$ would need to be to get this specific effective density.

## S5. MODEL DETAILS FOR THE POINT-CHARGE TOY PROBLEM

The toy dataset comprised of a gas of point particles interacting through pure electrostatic or dispersion interactions is built following the procedure discussed in the main text and in Ref. 11. For each structure we compute the atom centered spherical expansion where we use a single angular channel ($l = 0$), one radial channel for the optimized basis, and eight radial channels for the GTO basis. For the short range (SR) model we use a rather large cutoff of 9 Å and set the width of the Gaussian densities to $\sigma = 1$ Å. For the long-range (LR) LODE model we use an environment cut-off 0.1 Å and a Gaussian width of 0.6 Å. We perform simple ridge regression against the energy, using the implementation in Scikit-learn [13], with a regularizer of $1 \cdot 10^{-5}$. Given the linear nature of the model, we compute global descriptors of the structure by summing over all atom-centered descriptors within each structure, and apply the regression algorithm at the structure level.

## S6. COMPUTATIONAL DETAILS FOR THE DIMER DATASET

As discussed in the main text, we use a dataset based on the BioFragment Database (BFDb) [11, 14], that contains rigid-molecule binding curves for pairs of molecular fragments that are charged (C), polar (P) or apolar (A), which gives rise to six classes of dimer interactions.

### A. Reference energy calculations

We orient the dimers in a periodic cell with a length of 30 Å so that the connecting vector between the COMs of the two fragments points in the $(1, 1, 1)$ direction of the cell. Binding energies and forces are calculated using the Heyd, Scuseria, and Ernzerhof (HSE06) [15] hybrid functional together with a non-local many-body dispersion correction to handle the LR van der Waals (vdW) energy as implemented in the FHI-Aims package [16]. For the HSE06 functional, we split the exchange energy into 75 % Hartree-Fock and treat the remaining 25 % at the PBE level.

### B. Empirical interaction exponents

To extract the empirical decay exponents $p_{\mathrm{phys}}$ for the interaction energy from the data set we fit each binding curve individually to a linear function on a double logarithmic scale. The linear fit function has the form $f(r) = p_{\mathrm{phys}} \cdot r + b$, where $f$ can either be the energy $E$ or the magnitude of the molecular force $|F_{\mathrm{mol}}|$. The molecular force is defined as the sum of all forces acting on the atoms of each molecule (for a given dimer, the total forces on the two molecules are equal in magnitude and opposite in sign). Figure S6 shows all binding curves of a subset, i.e. CC for charge-charge, as

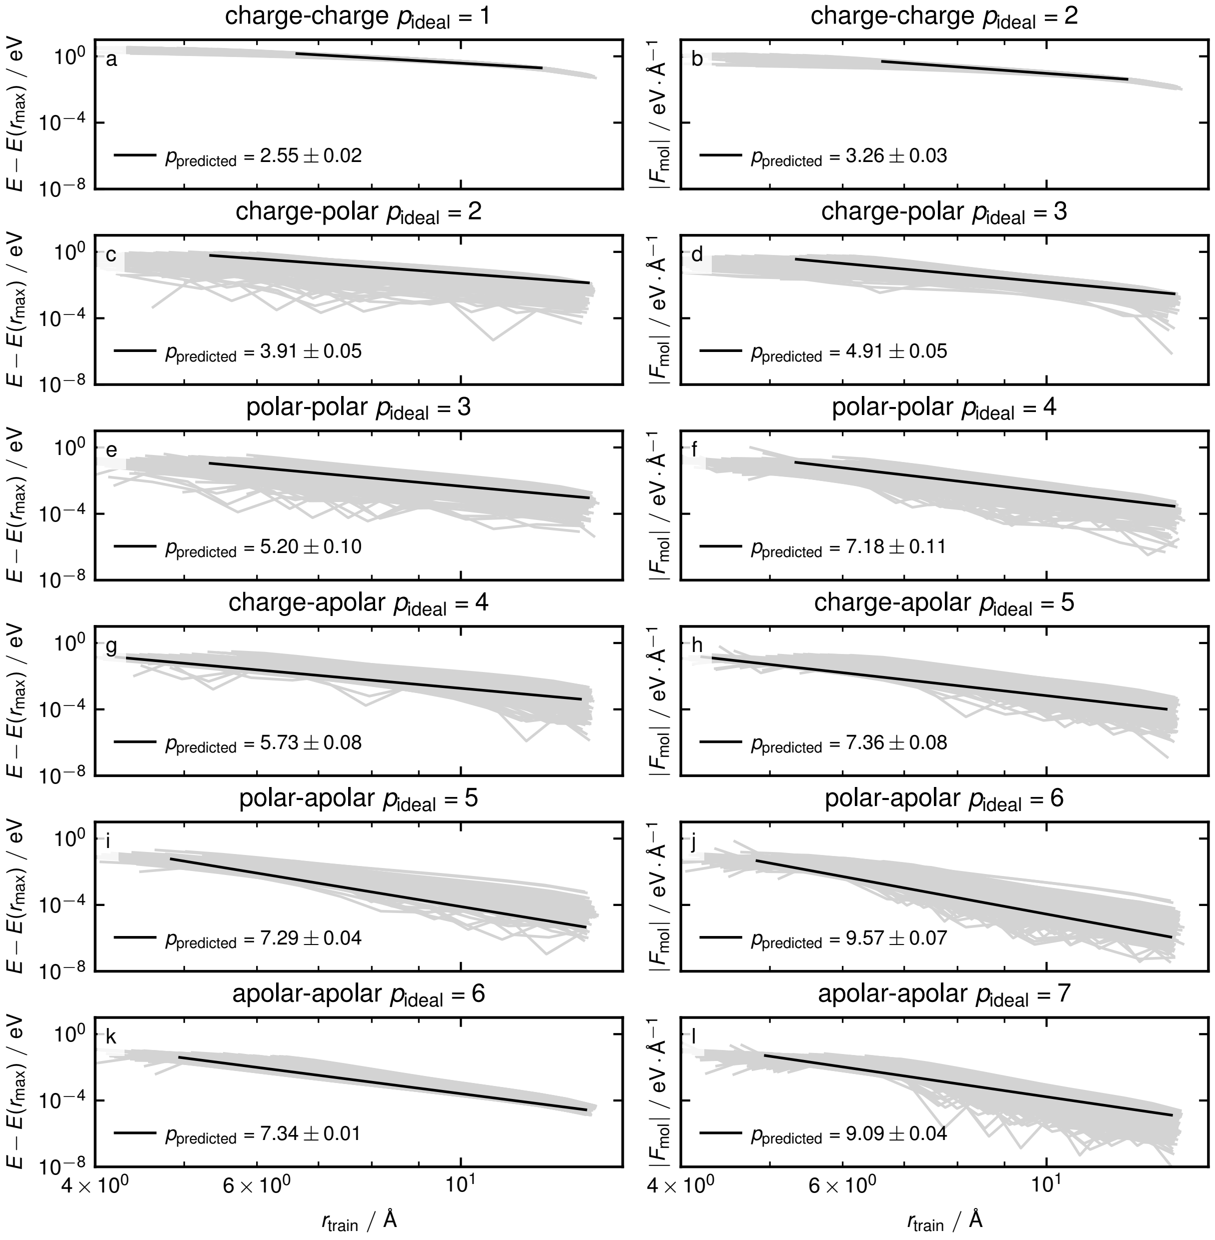


Figure S6. Dimer binding curves on a double logarithmic scale. Gray lines show the binding curves from the DFT simulation and solid black lines shows an example linear fit to a representative binding curve. Values in each figure legend indicate the mean and standard error for each $p_{phys}$. Each row of sub-panels shows binding curves for different subset of the dimers. Left columns: Binding energies $E - E(r_{max})$. For a better visualization all curves are shifted by the energy at the maximum separation $E(r_{max})$. Right columns: Absolute molecular force $|F_{mol}|$.

gray solid lines and one representative fit as a solid black line. The mean and standard error of each $p_{phys}$ is given in the legend of each sub-panel. We find that, for every type of interaction, the physical exponent is systematically higher compared to the ideal exponent $p_{ideal}$. This is an indication of the fact that molecules in the DFT simulation are not ideal point particles as assumed in the derivation of the ideal exponents. Spurious interactions between periodic replicas (especially for charged fragments), as well as noise in the binding energy at large distance (especially for weak interactions) contribute to this discrepancy.

### C. SOAP and LODE Hyperparameters

For the SR and the LR spherical expansions we use a cutoff/environment-cutoff of 3.0 Å. For the SR model we use a density Gaussian width of 0.3 Å, and expand the density on a basis including four angular channels, and six GTO-type radial basis channels. The density at the cutoff is smoothed using a shifted cosine switching function with a width of 0.5 Å. For the LR model we either use an optimal monomial basis containing one radial channel and one angular channel, or an extended monomial basis containing six radial and four angular channels, with the exponents determined according to the theoretical analysis in Section S2 F. For the LR desciptors we set the width of the Gaussian basis functions to 1 Å and we use no cosine switching function at the cutoff distance. From the atom centered spherical expansion coefficients of the density and the associated potential we construct the $\rho \otimes \rho \oplus \rho \otimes V_p$ multiscale power spectra according to [11].

### D. Linear Models: Separate Dimer Classes

We construct linear-regression models for each type of dimers, using global features obtained by summing over all atom-centered descriptors within each structure, supplemented by composition features that represent the stoichiometry of each structure through one-hot encoding of the atom types. During linear regression we use a very small regularizer of $2.2 \cdot 10^{-16}$ for the composition features and optimize the regularizer for the SR and LR features separately using a grid search. The grid ranges from $10^{-12}$ to $10^{3}$ and contains 20 logarithmically equispaced points. We find the optimal regularizer by minimizing the total RMSE of the energies and forces according to RMSE = $(\text{RMSE}_\text{energy} + \text{RMSE}_\text{force})/2$. Ridge regression is performed with the equisolve package, available at `https://github.com/lab-cosmo/equisolve`. Percentage RMSE are computed by normalizing the absolute RMSE values by the standard deviation of the binding energy of the training structures, computed separately for each dimer subset. As indicated in the main text, these are, for each subset: $\sigma$ =984 meV (CC); $\sigma$ =243 meV (CP); $\sigma$ =66 meV (PP); $\sigma$ =46 meV (CA); $\sigma$ =22 meV (PA); $\sigma$ =15 meV (PP).

### E. Atomic Force Errors

In Fig.S7 we compare the accuracy of the atomic force on the test set predicted by linear models using multiple monomial basis functions for the radial expansion. Similar to what shown in Fig.3b in the main text we compare different potential exponents $p = 1, 2, \ldots, 9$ and fit separately on each dimer fragment classe. As for the energy we find that all short-range models suffer from poor performance, and the inclusion of any LODE term leads to dramatic improvement in the test accuracy. However, the improvement is less pronounced than for the energies, and there is less-pronounced variation of the accuracy depending on the generalized LODE exponent, even though we find that the best potential exponent roughly corresponds to the ideal exponents for each dimer class.

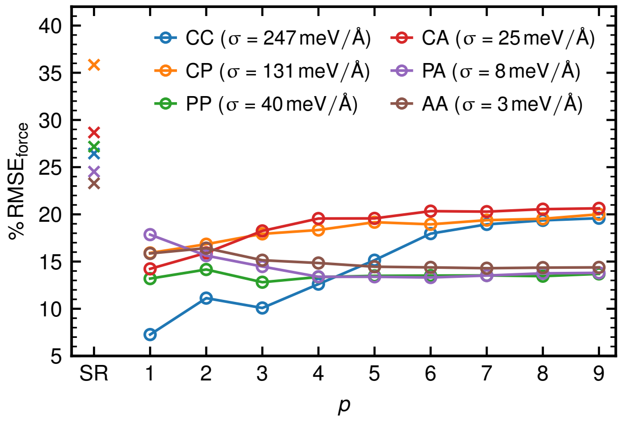


Figure S7. The figure shows the atomic force % RMSE as a function of the potential exponent $p$, similar to Fig. 3 in the main text.

### F. Test Errors for Different Training Cutoffs

We recall that the extrapolative learning exercise we perform involves predicting the long-range part of the binding curve, for $r > r_{\mathrm{train}}$, based on training on the part of the data set with $r \leq r_{\mathrm{train}}$ (where distances are defined relative to the minimal separation in the dataset for each dimer configuration). In Fig. S8 we show the % RMSE for the energies and forces for different subsets of the dataset as a function of the training cutoff $r_{\mathrm{train}}$ and the potential exponent $p$. We find that an increased training cutoff increases the accuracy on the test set. We note that due to the construction of our train/test split these curves are not usual learning curves. Contrary to the typical training exercises in which the number of test points remains constant, when the training cutoff is increased the number of training points increases while the number of test points decreases. This leads to a flattening of the RMSE curves as a function of the $r_{\mathrm{train}}$ for the shorter range interaction types like polar-polar, charge-apolar, polar-apolar and apolar-apolar. For these subsets their binding energy and force is almost zero if the two molecules are further apart then a few Å. Therefore, the learning accuracy will not increase for even larger $r_{\mathrm{train}}$ since the whole energy and force

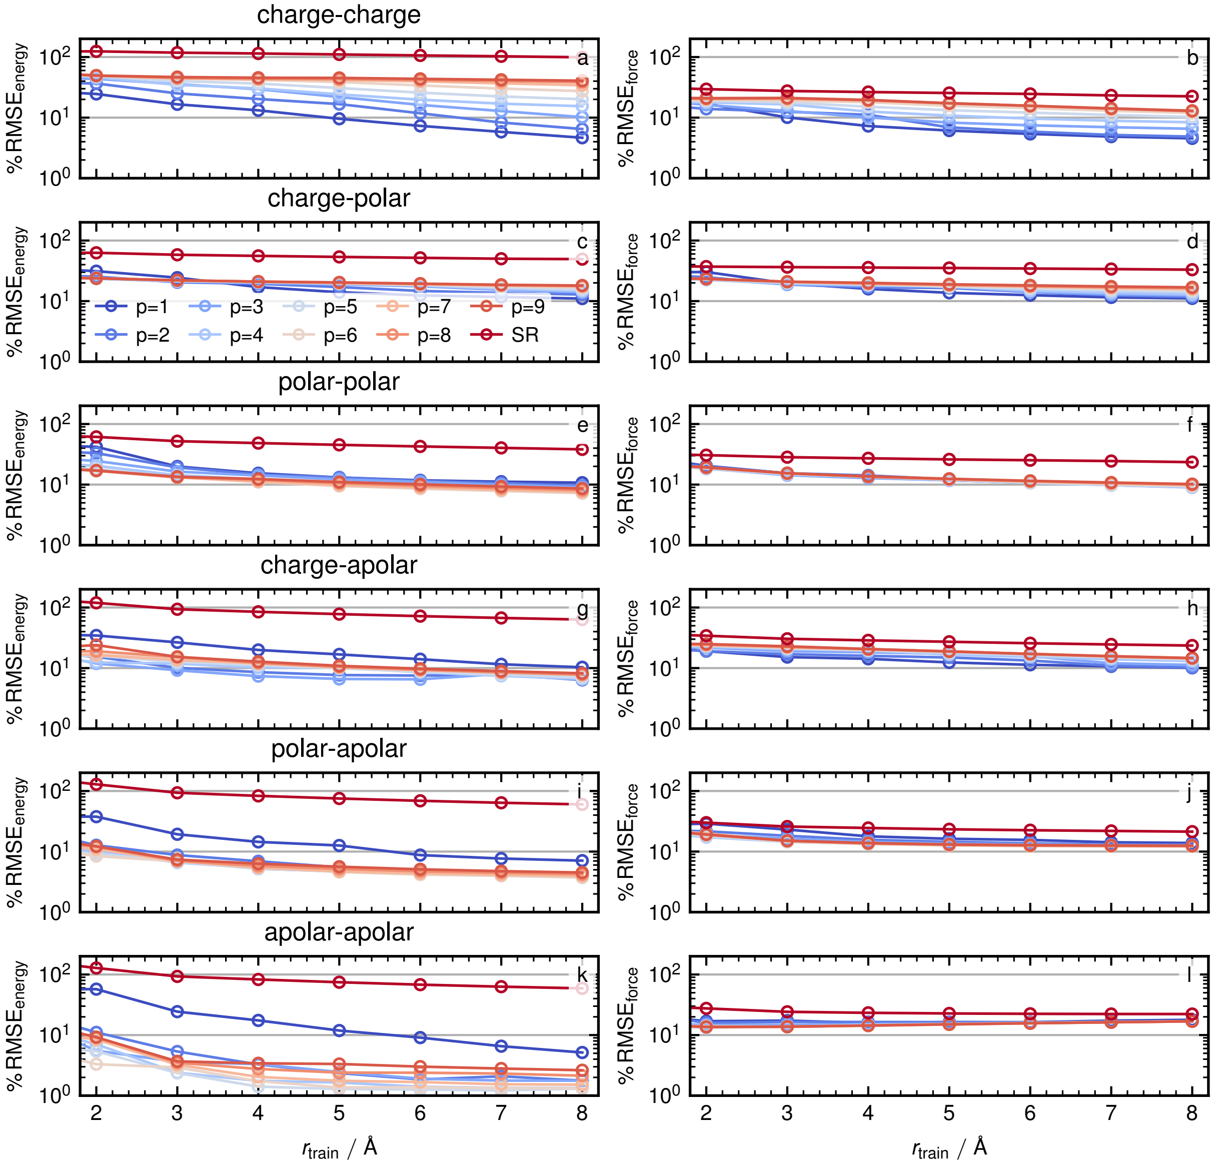


Figure S8. % RMSE for energies and forces for different dimer classes as a function of the training cutoff $r_{\mathrm{train}}$ and the potential exponent $p$. Subpanel titles indicate the corresponding dimer class. Left columns show $\%\,\mathrm{RMSE}_{\mathrm{energy}}$ while right columns show $\%\,\mathrm{RMSE}_{\mathrm{force}}$. Different colors indicate different potential exponents $p$ used in the generalized LODE descriptors.

can be fully described by the contributions of the isolated individual molecules. We also note that for the force RMSE we find only very little difference between the long and the short range models. This is due to the fact that the force on individual atoms is dominated by the force exerted by nearby atoms, which is usually not zero because of the fact that the binding curves are computed without relaxing the atoms at each interatomic separation.

From this discussion we conclude that the chosen train-test split of 4 Å, which we use in the rest of this work, is a reasonable choice since force curves have not already fully flattened out and the train set is sufficiently large for a physically-inspired model to be able to infer the asymptotic behavior of the interactions, and perform reasonable extrapolative predictions on the test set.

### G. Energy Errors for Combined Linear Models Using Non-Charged Fragments

In Fig.S9 we show the % RMSE of the energy for models trained on several dimer classes simultaneously. However, instead of training on the whole data set, we chose a subset excluding the charge-charge interactions (!CC, black open circles) or all dimer classes that contain some charged fragment (!C, gray open circles). The SR models show a very poor performance even though the slowest decaying $1/r$ interactions are left out. Comparing the black and the gray open circles we find that the model accuracy increases by a factor of two if all charged molecules are excluded from the model. This originates that for the remaining PP, PA and AP classes the standard deviation of the energies are very similar as we show in the legend of Fig.3b in the main text.

Comparing the potential exponent dependence for the training without the charge-charge fragments we find the best model for potential exponent is $p = 2$. This corresponds to the next slowest decaying interaction after CC, and therefore the largest contribution to the energy, that stems from the charge-polar fragments. For the training on the subset without any charged fragments we find a minimum around $p = 4$ which roughly corresponds to the ideal potential exponent of polar-polar interaction, which is 3. In addition, we find that the model accuracy is nearly independent in the range from $p = 2$ to $p = 6$, which is the range of the potential exponents for the PP, PA, and AA pairs. The weak dependence of the accuracy on the exponent for this subset is consistent with the similar weak dependence seen for the separate training exercises, and reflects the fact that (1) these weak interactions have a similar range of variability, so there is little gain in using an exponent optimized for one of the classes, and (2) the weaker interaction often show pronounced deviations from the ideal behavior (Fig. S6).

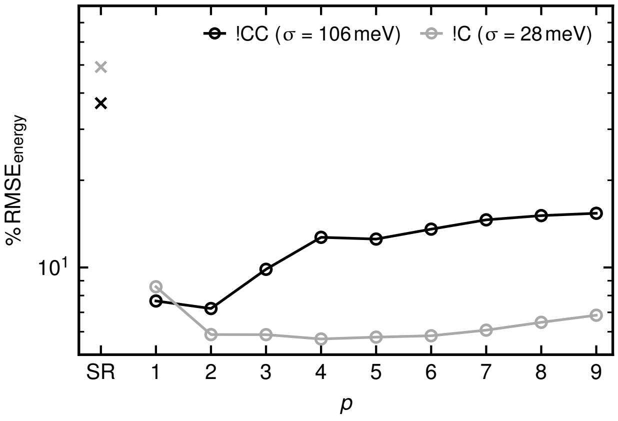


Figure S9. The figure shows the energy % RMSE for models trained on the energies of all dimer structures, up to a cutoff $r_{\text{train}} = 4$ Å, leaving out the CC fragments (!CC, in black) or all the dimers containing a charged residue (!C, in gray, including only PP, PA, AA dimers). The model details and training protocol are analogous to those used for Fig. 3 in the main text.

### H. Details of the Neural Network Models

We apply a multilayer perceptron neural network (NN) model to the concatenation of SR and LR descriptors at the level of individual environments, summing over the environments to determine the total energy of each structure, that is used as the target property. The NN uses three hidden layers each with 16 neurons. We use a sigmoid linear unit (SiLU) as activation function and perform a layer normalization for each layer. All models were trained using the Adam optimizer [17] as implemented in pytorch [18]. The learning rate is reduced by a factor of 0.8 every 1000 epochs if the validation loss reaches a plateau. Means and errors of the RMSE's are obtained from five independent training runs. In Fig. S10 we show a bar plot analogous to Fig. 4 in the main text, displaying the % RMSE on the train set for energies and forces for the neural network (NN) models. The figure shows that the additional flexibility

afforded by a NN architecture allows to improve the accuracy in the interpolative regime, but is not able to improve the extrapolative performance, that requires a physical prior.

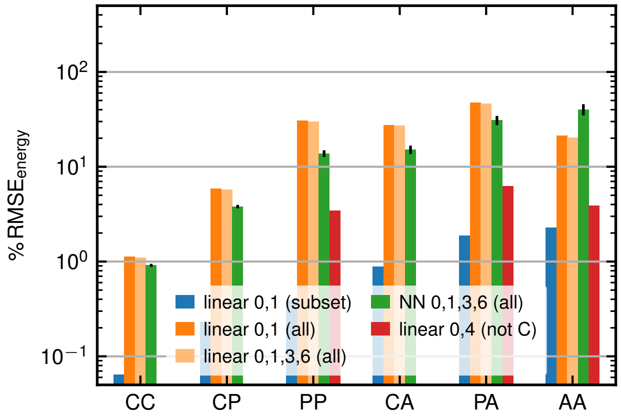


Figure S10. % RMSE on the train set for the energies for the different subsets of the dimers. The vertical scale and color coding match those used in Fig. 4 in the main text. Blue bars show the RMSE of models using a single $p = 1$ LODE exponent. Orange and light orange bars show linear models fit to the whole data set. Green bars show a fit to the whole data set with a non-linear neural network model. Red bars correspond to a linear model restricted to non-charged fragments.

## I. Absolute Eenergy Errors for Different Subsets

In Fig. S11a we plot the absolute RMSE in eV based on the data of Fig. 4 in the main text which shows the relative error on the test set. Figure. S11b shows the absolute error on the training set based on the results shown in Fig. S10. The figure shows that for a training on the whole dataset the absolute errors on all subsets are comparable, and the main challenge in improving the relative accuracy for the weaker interactions is due the the discrepancy between the energy scale of different long-range effects.

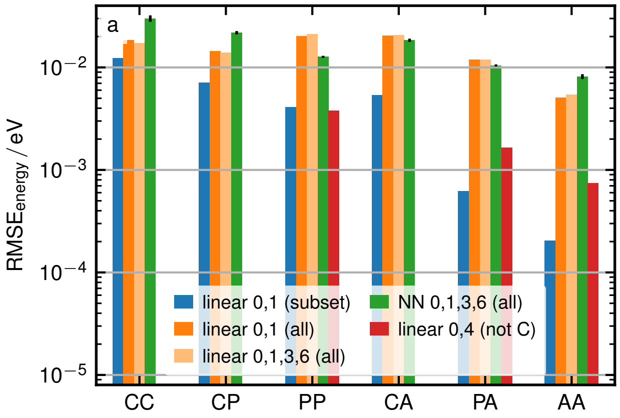


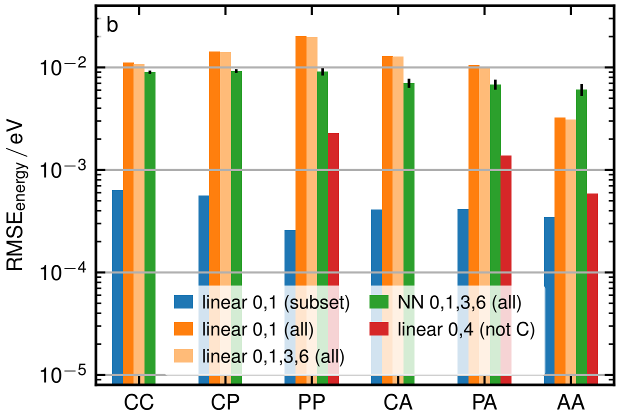


Figure S11. Absolute RMSE in eV on the test a and the train a set for the energies for the different subsets. Blue bars show the RMSE of models using a single $p = 1$ LODE exponent Orange and light orange bars show linear models fit to the whole data set. Green bars show a fit to the whole data set with a non-linear neural network model. Red bars correspond to a linear model restricted to non-charged fragments.

## S7. FLEXIBILITY OF POWER-LAW FITS

In this section we show a simple example to illustrate how, given a sufficiently flexible functional form, different types of asymptotic behavior can be achieved using a single potential exponent for the LR features. We consider the following toy model in one dimension: We aim to fit a target function $f(x) = 1/|x|^p$ for fixed $p$. To do so, we use 6 "atoms" with $x$ coordinates $x \in (-2.5, -1.3, -0.4, 0.5, 1.4, 2.2)$, i.e. atoms around the origin with average distance on the order of 1 roughly corresponding to interatomic distances in Å. We then assume that each of the $i = 1, \ldots, 6$

points generates a $1/|x|^{p'}$ potential, where $p' \neq p$ is different from the true exponent, and with "charges" $q_i$ that can be fitted to the data. Thus, we obtain the fitting function

$$\tilde{f}(x) = \sum_{i=1}^{6} \frac{q_i}{|x - x_i|^{p'}}. \tag{S89}$$

In Fig. S12 a and b, we try to fit a true underlying function $f(x) = 1/|x|$ (i.e. $p = 1$) using a superposition of six $1/|x|^3$ functions (i.e. $p' = 3$). We compare the true function (black solid line) against the obtained least squares fit (red dashed line), where the fit was performed such as to minimize the squared error

$$\text{Loss} = \int_{x_{\min}}^{x_{\max}} |f(x) - \tilde{f}(x)|^2 \, \mathrm{d}x, \tag{S90}$$

where the fitting interval was chosen to be $[x_{\min}, x_{\max}] = [5, 10]$.

In Fig. S12a, we can see that in this fitting interval, the six $1/|x|^3$ functions lead to an essentially perfect fit of the true underlying $1/|x|$ potential. However, as we move to figure b, and observe how the fit performs against the true behavior for distances beyond the fitting interval, we can see that fit is not truly capturing the LR $1/|x|$ behavior. In fact, as is expected, the asymptotic behavior of $\tilde{f}$ as $x \to \infty$ does indeed approach a $1/|x|^3$ form matching the terms in the fitting function.

In Fig.S12c and d, we repeat the same exercise but with exponents flipped: the true underlying function (black solid line) is given by $f(x) = 1/|x|^3$, which is fitted by the superposition of six functions decaying as $1/|x|$ (red dashed line). We can again see that the fit is excellent in the fitting interval $x = [5, 10]$ (Fig. S12c). A key difference to the previous case, however, is that also in the extrapolative regime d, the fit still remains accurate up to significantly larger distances. In fact, as was shown in much more generality in the section on the multipole expansion S1, it is possible for a superposition of $1/|x|$ potentials to generate a function with an asymptotic behavior of $1/|x|^3$. To provide a simpler example that only requires knowledge about the geometric series, we can use that for $x \to +\infty$

$$\frac{1}{|x \pm a|} = \frac{1}{x \pm a} = \frac{1}{x} \frac{1}{1 \pm \frac{a}{x}} = \frac{1}{x} \left( 1 \mp \frac{a}{x} + \frac{a^2}{x^2} \mp \frac{a^3}{x^4} + \right) = \frac{1}{x} \mp \frac{a}{x^2} + \frac{a^2}{x^3} \mp \frac{a^3}{x^4} + \dots \tag{S91}$$

and thus

$$\frac{1}{|x + a|} + \frac{1}{|x - a|} = 2\frac{a}{x^2} + 2\frac{a^3}{x^4} + \dots \tag{S92}$$

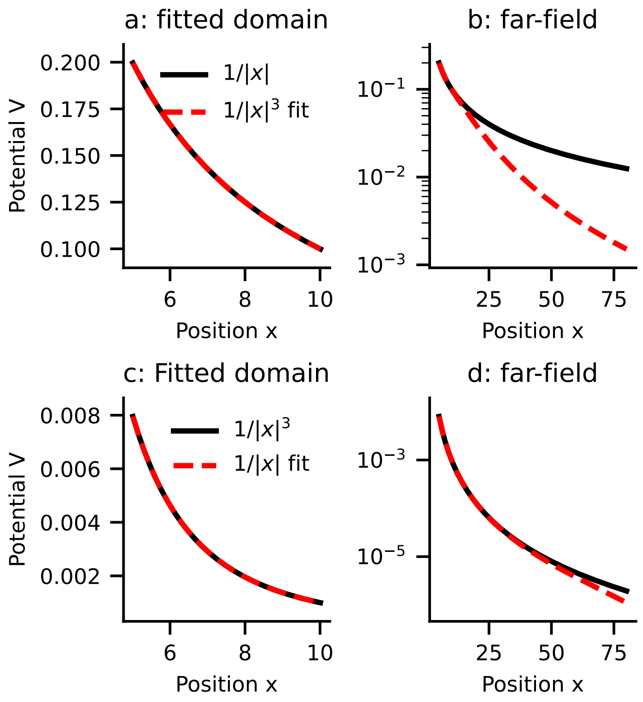


Figure S12. Fitting power law decaying potential with different exponents. Black line shows the to be fitted power law $1/r$ and red dashed line show a fit with a $1/r^3$ power law.

showing that a superposition of two functions decaying as $1/|x|$ can indeed generate a function decaying as $1/|x|^2$, if the relative weights (here, we assumed that the two potentials have the same "charge" / prefactor) and offsets (here: $+a$ and $-a$) lead to a perfect cancellation of the leading $1/|x|$ term. Superpositions of three such functions can then in principle lead to asymptotic $1/|x|^3$ behavior, etc. While possible in principle, this requires a perfect cancellation of terms, which is why the fit in S12(d) does deviate from the perfect $1/|x|^3$ behavior at very large distances.

In summary, we can see that restricted to intermediate distances, one can in principle fit any exponent $p$ from any other reasonably close exponent $p'$, which does not mean that the true far-field behavior is captured. This lack of extrapolation capability for large distances can either be due to fundamental limitations, namely if $p < p'$, or due to the high numerical accuracy that is required to obtain a perfect cancellation of leading order terms for $p > p'$.

We can also flip the story around: if we are only given a superposition of $1/|x|^{p'}$ potentials, e.g. the red dashed lines in the figures S12a and c, and want to find the best $q/|x|^p$ fit for suitable parameters $q$ and $p$, the exponent we obtain from the fit will typically not be the correct exponent $p'$ unless we can work in the true $x \to \infty$ limit and no cancellations as discussed above happen (which, in the absence of special symmetries, should only occur with a probability of zero). This shows how the very concept of an "exponent" characterizing a potential can be quite subtle when working with dense systems and a limited dataset.

---


[1] J. D. Jackson, *Classical Electrodynamics Third Edition*, 3rd ed. (Wiley, New York, 1998).

[2] F. Musil, A. Grisafi, A. P. Bartók, C. Ortner, G. Csányi, and M. Ceriotti, Physics-Inspired Structural Representations for Molecules and Materials, Chemical Reviews **121**, 9759 (2021), publisher: American Chemical Society.

[3] A. P. Bartók, M. C. Payne, R. Kondor, and G. Csányi, Gaussian Approximation Potentials: The Accuracy of Quantum Mechanics, without the Electrons, Physical Review Letters **104**, 136403 (2010), publisher: American Physical Society.

[4] A. P. Bartók, R. Kondor, and G. Csányi, On representing chemical environments, Physical Review B **87**, 184115 (2013), publisher: American Physical Society.

[5] J. Behler and M. Parrinello, Generalized Neural-Network Representation of High-Dimensional Potential-Energy Surfaces, Physical Review Letters **98**, 146401 (2007), publisher: American Physical Society.

[6] R. Drautz, Atomic cluster expansion for accurate and transferable interatomic potentials, Phys. Rev. B **99**, 014104 (2019).

[7] A. Grisafi and M. Ceriotti, Incorporating long-range physics in atomic-scale machine learning, The Journal of Chemical Physics **151**, 204105 (2019), publisher: American Institute of Physics.

[8] B. R. A. Nijboer and F. W. De Wette, On the calculation of lattice sums, Physica **23**, 309 (1957).

[9] D. E. Williams, Accelerated convergence of crystal-lattice potential sums, Acta Crystallographica Section A: Crystal Physics, Diffraction, Theoretical and General Crystallography **27**, 452 (1971), number: 5 Publisher: International Union of Crystallography.

[10] D. E. Williams, Accelerated Convergence Treatment of R-n Lattice Sums, Crystallography Reviews **2**, 3 (1989), publisher: Taylor & Francis _eprint: https://doi.org/10.1080/08893118908032944.

[11] A. Grisafi, J. Nigam, and M. Ceriotti, Multi-scale approach for the prediction of atomic scale properties, Chemical Science **12**, 2078 (2021), publisher: Royal Society of Chemistry.

[12] A. Grisafi, D. M. Wilkins, G. Csányi, and M. Ceriotti, Symmetry-Adapted Machine Learning for Tensorial Properties of Atomistic Systems, Physical Review Letters **120**, 036002 (2018), publisher: American Physical Society.

[13] F. Pedregosa, G. Varoquaux, A. Gramfort, V. Michel, B. Thirion, O. Grisel, M. Blondel, P. Prettenhofer, R. Weiss, V. Dubourg, J. Vanderplas, A. Passos, D. Cournapeau, M. Brucher, M. Perrot, and E. Duchesnay, Scikit-learn: Machine learning in Python, Journal of Machine Learning Research **12**, 2825 (2011).

[14] L. A. Burns, J. C. Faver, Z. Zheng, M. S. Marshall, D. G. A. Smith, K. Vanommeslaeghe, A. D. MacKerell, K. M. Merz, and C. D. Sherrill, The BioFragment Database (BFDb): An open-data platform for computational chemistry analysis of noncovalent interactions, J. Chem. Phys. **147**, 161727 (2017).

[15] J. Heyd, G. E. Scuseria, and M. Ernzerhof, Hybrid functionals based on a screened Coulomb potential, The Journal of Chemical Physics **118**, 8207 (2003).

[16] V. Blum, R. Gehrke, F. Hanke, P. Havu, V. Havu, X. Ren, K. Reuter, and M. Scheffler, Ab initio molecular simulations with numeric atom-centered orbitals, Computer Physics Communications **180**, 2175 (2009).

[17] D. P. Kingma and J. Ba, Adam: A Method for Stochastic Optimization (2017), arxiv:1412.6980 [cs].

[18] A. Paszke, S. Gross, F. Massa, A. Lerer, J. Bradbury, G. Chanan, T. Killeen, Z. Lin, N. Gimelshein, L. Antiga, A. Desmaison, A. Köpf, E. Yang, Z. DeVito, M. Raison, A. Tejani, S. Chilamkurthy, B. Steiner, L. Fang, J. Bai, and S. Chintala, PyTorch: An Imperative Style, High-Performance Deep Learning Library (2019), arxiv:1912.01703 [cs, stat].
